# Supplementary material for: Theory of polar domains in moir\'e heterostructures
Source: arXiv:2203.01979 source file (2022-09-19)
Supplement: Supplementary file 1 [file SI.pdf]

# SUPPLEMENTARY INFORMATION
# Theory of polar domains in moiré heterostructures

Daniel Bennett[1,2,*]

[1]*Theory of Condensed Matter, Cavendish Laboratory, Department of Physics, J J Thomson Avenue, Cambridge CB3 0HE, United Kingdom*
[2]*Physique Théorique des Matériaux, QMAT, CESAM, University of Liège, B-4000 Sart-Tilman, Belgium*
(Dated: March 3, 2022)

## I. TABLES AND FIGURES SUMMARIZING RESULTS FROM FIRST-PRINCIPLES CALCULATIONS

| Stacking | Quantity | $\phi_0$ | $\phi_1^{\text{even}}$ | $\phi_2^{\text{even}}$ | $\phi_3^{\text{even}}$ | $\phi_1^{\text{odd}}$ | $\phi_2^{\text{odd}}$ | $\phi_3^{\text{odd}}$ |
|---|---|---|---|---|---|---|---|---|
| 3R | $\mathcal{V}_{\text{stack}}$ (eV) | -0.154 | 0.010 | -0.0008 | 0.0 | 0.0 | 0.0 | 0.0 |
| | $d_0$ (Å) | 3.250 | 0.0655 | -0.00246 | -0.00118 | 0.0 | 0.0 | 0.0 |
| | $\alpha_0$ (Å$^3$) | 22.139 | -0.122 | -0.0342 | -0.00970 | 0.0 | 0.0 | 0.0 |
| | $\alpha_1$ (Å$^3$) | 3.470 | 0.512 | 0.0781 | 0.0377 | 0.0 | 0.0 | 0.0 |
| | $p_0 \times 10^2$ (eÅ) | 0.0 | 0.0 | 0.0 | 0.0 | -0.203 | 0.0 | 0.0156 |
| | $P_0 \times 10^5$ (eÅ$^{-2}$) | 0.0 | 0.0 | 0.0 | 0.0 | -11.629 | 0.0 | 1.004 |
| 2H | $\mathcal{V}_{\text{stack}}$ (eV) | -0.153 | -0.00342 | -0.0005 | 0.0002 | -0.00651 | 0.0 | -0.0002 |
| | $d_0$ (Å) | 3.251 | -0.0248 | -0.00220 | 0.0006 | -0.0473 | 0.0 | -0.0007 |
| | $\alpha_0$ (Å$^3$) | 22.166 | 0.0345 | -0.0302 | 0.0158 | 0.187 | 0.0 | -0.0165 |
| | $\alpha_1$ (Å$^3$) | 3.334 | -0.155 | -0.0634 | 0.0 | -0.354 | 0.0 | 0.0 |
| | $p_0 \times 10^2$ (eÅ) | 0.0 | 0.0 | 0.0 | 0.0 | 0.0 | 0.0 | 0.0 |
| | $P_0 \times 10^5$ (eÅ$^{-2}$) | 0.0 | 0.0 | 0.0 | 0.0 | 0.0 | 0.0 | 0.0 |

TABLE I. Fitting parameters for bilayer hBN.

* db729@cantab.ac.uk

| Stacking | Quantity | $\phi_0$ | $\phi_1^{even}$ | $\phi_2^{even}$ | $\phi_3^{even}$ | $\phi_1^{odd}$ | $\phi_2^{odd}$ | $\phi_3^{odd}$ |
|---|---|---|---|---|---|---|---|---|
| 3R | $\mathcal{V}_{stack}$ (eV) | -0.219 | 0.0239 | -0.00519 | 0.00158 | 0.0 | 0.0 | 0.0 |
| | $d_0$ (Å) | 6.332 | 0.165 | -0.0306 | -0.0104 | 0.0 | 0.0 | 0.0 |
| | $\alpha_0$ (Å$^3$) | 93.623 | 1.410 | -0.246 | -0.0903 | 0.0 | 0.0 | 0.0 |
| | $\alpha_1$ (Å$^3$) | 52.848 | 2.659 | -0.980 | -0.161 | 0.0 | 0.0 | 0.0 |
| | $p_0 \times 10^2$ (eÅ) | 0.0 | 0.0 | 0.0 | 0.0 | 0.134 | 0.0 | -0.0288 |
| | $P_0 \times 10^5$ (eÅ$^{-2}$) | 0.0 | 0.0 | 0.0 | 0.0 | 2.532 | 0.0 | -0.5808 |
| 2H | $\mathcal{V}_{stack}$ (eV) | -0.217 | -0.00614 | -0.00412 | 0.00121 | -0.0199 | 0.0 | 0.0 |
| | $d_0$ (Å) | 6.345 | -0.0647 | -0.0250 | 0.0 | 0.132 | 0.0 | -0.0108 |
| | $\alpha_0$ (Å$^3$) | 93.711 | -0.563 | -0.201 | 0.00515 | -1.129 | 0.0 | -0.0956 |
| | $\alpha_1$ (Å$^3$) | 53.153 | -0.952 | -0.756 | 0.0 | -2.064 | 0.0 | 0.0 |
| | $p_0 \times 10^2$ (eÅ) | 0.0 | 0.0 | 0.0 | 0.0 | 0.0 | 0.0 | 0.0 |
| | $P_0 \times 10^5$ (eÅ$^{-2}$) | 0.0 | 0.0 | 0.0 | 0.0 | 0.0 | 0.0 | 0.0 |

TABLE II. Fitting parameters for bilayer $MoS_2$.

| Stacking | Quantity | $\phi_0$ | $\phi_1^{even}$ | $\phi_2^{even}$ | $\phi_3^{even}$ | $\phi_1^{odd}$ | $\phi_2^{odd}$ | $\phi_3^{odd}$ |
|---|---|---|---|---|---|---|---|---|
| 3R | $\mathcal{V}_{stack}$ (eV) | -0.212 | 0.212 | -0.00412 | -0.00151 | 0.0 | 0.0 | 0.0 |
| | $d_0$ (Å) | 6.759 | 0.148 | -0.0185 | -0.00794 | 0.0 | 0.0 | 0.0 |
| | $\alpha_0$ (Å$^3$) | 110.111 | 1.388 | -0.168 | -0.0739 | 0.0 | 0.0 | |
| | $\alpha_1$ (Å$^3$) | 62.581 | 1.944 | -0.381 | -0.100 | 0.0 | 0.0 | 0.0 |
| | $p_0 \times 10^2$ (eÅ) | 0.0 | 0.0 | 0.0 | 0.0 | 0.0884 | 0.0 | -0.0156 |
| | $P_0 \times 10^5$ (eÅ$^{-2}$) | 0.0 | 0.0 | 0.0 | 0.0 | 1.421 | 0.0 | -0.267 |
| 2H | $\mathcal{V}_{stack}$ (eV) | -0.210 | -0.00607 | -0.00327 | 0.00102 | -0.0173 | 0.0 | 0.0 |
| | $d_0$ (Å) | 6.767 | -0.0548 | -0.0159 | 0.00588 | -0.118 | 0.0 | -0.00576 |
| | $\alpha_0$ (Å$^3$) | 11.0281 | -0.518 | -0.146 | -0.0547 | -1.108 | 0.0 | -0.0537 |
| | $\alpha_1$ (Å$^3$) | 62.831 | -0.652 | -0.256 | 0.0744 | -1.488 | 0.0 | -0.080 |
| | $p_0 \times 10^2$ (eÅ) | 0.0 | 0.0 | 0.0 | 0.0 | 0.0 | 0.0 | 0.0 |
| | $P_0 \times 10^5$ (eÅ$^{-2}$) | 0.0 | 0.0 | 0.0 | 0.0 | 0.0 | 0.0 | 0.0 |

TABLE III. Fitting parameters for bilayer $MoSe_2$.

| Stacking | Quantity | $\phi_0$ | $\phi_1^{\text{even}}$ | $\phi_2^{\text{even}}$ | $\phi_3^{\text{even}}$ | $\phi_1^{\text{odd}}$ | $\phi_2^{\text{odd}}$ | $\phi_3^{\text{odd}}$ |
|---|---|---|---|---|---|---|---|---|
| 3R | $\mathcal{V}_{\text{stack}}$ (eV) | -0.224 | 0.0239 | -0.00478 | -0.00168 | 0.0 | 0.0 | 0.0 |
| | $d_0$ (Å) | 6.361 | 0.156 | -0.0239 | -0.00844 | 0.0 | 0.0 | 0.0 |
| | $\alpha_0$ (Å$^3$) | 94.213 | 1.361 | -0.205 | -0.0737 | 0.0 | 0.0 | |
| | $\alpha_1$ (Å$^3$) | 54.719 | 1.878 | -0.576 | -0.0951 | 0.0 | 0.0 | 0.0 |
| | $p_0 \times 10^2$ (eÅ) | 0.0 | 0.0 | 0.0 | 0.0 | 0.131 | 0.0 | -0.0259 |
| | $P_0 \times 10^5$ (eÅ$^{-2}$) | 0.0 | 0.0 | 0.0 | 0.0 | 2.439 | 0.0 | -0.512 |
| 2H | $\mathcal{V}_{\text{stack}}$ (eV) | -0.222 | -0.00624 | -0.00389 | 0.00132 | -0.0199 | 0.0 | 0.0 |
| | $d_0$ (Å) | 6.371 | -0.0571 | -0.0191 | 0.00310 | -0.127 | 0.0 | -0.00725 |
| | $\alpha_0$ (Å$^3$) | 94.341 | -0.509 | -0.165 | 0.0251 | -1.110 | 0.0 | -0.0643 |
| | $\alpha_1$ (Å$^3$) | 54.943 | -0.395 | -0.383 | 0.0 | -1.507 | 0.0 | 0.0 |
| | $p_0 \times 10^2$ (eÅ) | 0.0 | 0.0 | 0.0 | 0.0 | 0.0 | 0.0 | 0.0 |
| | $P_0 \times 10^5$ (eÅ$^{-2}$) | 0.0 | 0.0 | 0.0 | 0.0 | 0.0 | 0.0 | 0.0 |

TABLE IV. Fitting parameters for bilayer $WS_2$.

| Stacking | Quantity | $\phi_0$ | $\phi_1^{\text{even}}$ | $\phi_2^{\text{even}}$ | $\phi_3^{\text{even}}$ | $\phi_1^{\text{odd}}$ | $\phi_2^{\text{odd}}$ | $\phi_3^{\text{odd}}$ |
|---|---|---|---|---|---|---|---|---|
| 3R | $\mathcal{V}_{\text{stack}}$ (eV) | -0.205 | 0.0201 | -0.00395 | -0.00141 | 0.0 | 0.0 | 0.0 |
| | $d_0$ (Å) | 6.710 | 0.146 | -0.0110 | -0.00896 | 0.0 | 0.0 | 0.0 |
| | $\alpha_0$ (Å$^3$) | 110.379 | 1.376 | -0.183 | -0.0853 | 0.0 | 0.0 | |
| | $\alpha_1$ (Å$^3$) | 63.449 | 1.810 | -0.320 | -0.131 | 0.0 | 0.0 | 0.0 |
| | $p_0 \times 10^2$ (eÅ) | 0.0 | 0.0 | 0.0 | 0.0 | 0.0915 | 0.0 | -0.0153 |
| | $P_0 \times 10^5$ (eÅ$^{-2}$) | 0.0 | 0.0 | 0.0 | 0.0 | 1.455 | 0.0 | -0.259 |
| 2H | $\mathcal{V}_{\text{stack}}$ (eV) | -0.204 | -0.00505 | -0.00318 | 0.00105 | -0.0171 | 0.0 | 0.0 |
| | $d_0$ (Å) | 6.808 | -0.0494 | -0.0174 | 0.00520 | -0.120 | 0.0 | -0.00596 |
| | $\alpha_0$ (Å$^3$) | 110.541 | -0.472 | -0.161 | 0.0479 | -1.135 | 0.0 | -0.0563 |
| | $\alpha_1$ (Å$^3$) | 63.675 | -0.529 | -0.246 | 0.0684 | -1.474 | 0.0 | -0.0825 |
| | $p_0 \times 10^2$ (eÅ) | 0.0 | 0.0 | 0.0 | 0.0 | 0.0 | 0.0 | 0.0 |
| | $P_0 \times 10^5$ (eÅ$^{-2}$) | 0.0 | 0.0 | 0.0 | 0.0 | 0.0 | 0.0 | 0.0 |

TABLE V. Fitting parameters for bilayer $WSe_2$.

| Stacking | Quantity | $\phi_0$ | $\phi_1^{\text{even}}$ | $\phi_2^{\text{even}}$ | $\phi_3^{\text{even}}$ | $\phi_1^{\text{odd}}$ | $\phi_2^{\text{odd}}$ | $\phi_3^{\text{odd}}$ |
|---|---|---|---|---|---|---|---|---|
| 3R | $\mathcal{V}_{\text{stack}}$ (eV) | -0.129 | 0.0226 | -0.00423 | -0.00151 | -0.00135 | 0.0 | 0.0 |
| | $d_0$ (Å) | 6.552 | 0.151 | -0.0208 | -0.00765 | -0.00547 | 0.0 | 0.0 |
| | $\alpha_0$ (Å$^3$) | 100.494 | 1.297 | -0.172 | -0.0651 | -0.0467 | 0.0 | -0.00111 |
| | $\alpha_1$ (Å$^3$) | 55.594 | 2.001 | -0.330 | -0.0950 | -0.0678 | 0.0 | -0.0141 |
| | $p_0 \times 10^2$ (eÅ) | 0.908 | -0.111 | 0.0187 | 0.00595 | 0.0109 | 0.0 | -0.0184 |
| | $P_0 \times 10^5$ (eÅ$^{-2}$) | 15.377 | -2.120 | 0.413 | 0.127 | 1.917 | 0.0 | -0.345 |
| 2H | $\mathcal{V}_{\text{stack}}$ (eV) | -0.127 | -0.00662 | -0.00340 | 0.00124 | -0.0185 | 0.0 | 0.0 |
| | $d_0$ (Å) | 6.558 | -0.0544 | -0.0172 | 0.00373 | -0.124 | 0.0 | -0.00656 |
| | $\alpha_0$ (Å$^3$) | 100.611 | -0.466 | -0.143 | 0.0320 | -1.068 | 0.0 | -0.0555 |
| | $\alpha_1$ (Å$^3$) | 55.708 | -0.781 | -0.273 | 0.0460 | -1.601 | 0.0 | -0.0839 |
| | $p_0 \times 10^2$ (eÅ) | 0.909 | 0.0473 | 0.0150 | -0.00259 | 0.0862 | 0.0 | 0.00626 |
| | $P_0 \times 10^5$ (eÅ$^{-2}$) | 15.353 | 0.909 | 0.329 | -0.0595 | 1.728 | 0.0 | 0.127 |

TABLE VI. Fitting parameters for bilayer $MoS_2$/MoSe2.

| Stacking | Quantity | $\phi_0$ | $\phi_1^{\text{even}}$ | $\phi_2^{\text{even}}$ | $\phi_3^{\text{even}}$ | $\phi_1^{\text{odd}}$ | $\phi_2^{\text{odd}}$ | $\phi_3^{\text{odd}}$ |
|---|---|---|---|---|---|---|---|---|
| 3R | $\mathcal{V}_{\text{stack}}$ (eV) | -0.130 | 0.0224 | -0.00456 | -0.00150 | -0.00190 | 0.0 | 0.0 |
| | $d_0$ (Å) | 6.573 | 0.149 | -0.0216 | -0.00851 | -0.00684 | 0.0 | 0.00106 |
| | $\alpha_0$ (Å$^3$) | 100.527 | 1.289 | -0.178 | -0.0738 | -0.0644 | 0.0 | 0.00939 |
| | $\alpha_1$ (Å$^3$) | 56.255 | 2.124 | -0.445 | -0.108 | -0.0410 | 0.0 | 0.0205 |
| | $p_0 \times 10^2$ (eÅ) | 0.762 | -0.0925 | 0.0162 | 0.00528 | 0.114 | 0.0 | -0.0205 |
| | $P_0 \times 10^5$ (eÅ$^{-2}$) | 12.780 | -1.820 | 0.354 | 0.110 | 1.980 | 0.0 | -0.379 |
| 2H | $\mathcal{V}_{\text{stack}}$ (eV) | -0.128 | -0.00596 | -0.00370 | 0.00126 | -0.0187 | 0.0 | 0.0 |
| | $d_0$ (Å) | 6.583 | -0.0517 | -0.0191 | 0.00500 | -0.123 | 0.0 | -0.00661 |
| | $\alpha_0$ (Å$^3$) | 100.654 | -0.453 | -0.160 | 0.0425 | -1.070 | 0.0 | -0.0579 |
| | $\alpha_1$ (Å$^3$) | 56.460 | -0.705 | -0.349 | 0.0746 | -1.711 | 0.0 | -0.0820 |
| | $p_0 \times 10^2$ (eÅ) | 0.763 | 0.0348 | 0.0130 | -0.00310 | 0.0773 | 0.0 | 0.00526 |
| | $P_0 \times 10^5$ (eÅ$^{-2}$) | 12.762 | 0.667 | 0.283 | -0.0682 | 1.521 | 0.0 | 0.104 |

TABLE VII. Fitting parameters for bilayer $WS_2$/WSe2.

| Stacking | Quantity | $\phi_0$ | $\phi_1^{\rm even}$ | $\phi_2^{\rm even}$ | $\phi_3^{\rm even}$ | $\phi_1^{\rm odd}$ | $\phi_2^{\rm odd}$ | $\phi_3^{\rm odd}$ |
|---|---|---|---|---|---|---|---|---|
| 3R | $\mathcal{V}_{\rm stack}$ (eV) | -0.221 | 0.0240 | -0.00493 | -0.00159 | 0.0 | 0.0 | 0.0 |
| | $d_0$ (Å) | 6.345 | 0.160 | -0.0270 | -0.00926 | 0.0 | 0.0 | 0.0 |
| | $\alpha_0$ (Å$^3$) | 93.882 | 1.392 | -0.223 | -0.0821 | 0.0133 | 0.0 | 0.0100 |
| | $\alpha_1$ (Å$^3$) | 53.706 | 2.301 | -0.773 | -0.134 | 0.116 | 0.0 | -0.667 |
| | $p_0 \times 10^2$ (eÅ) | 0.0485 | -0.0351 | 0.00938 | 0.00342 | 0.132 | 0.0 | -0.0276 |
| | $P_0 \times 10^5$ (eÅ$^{-2}$) | 0.903 | -0.655 | 0.189 | 0.0644 | 2.482 | 0.0 | -0.549 |
| 2H | $\mathcal{V}_{\rm stack}$ (eV) | -0.219 | -0.00619 | -0.00397 | 0.00129 | -0.0200 | 0.0 | 0.0 |
| | $d_0$ (Å) | 6.357 | -0.0592 | -0.0216 | 0.00207 | -0.130 | 0.0 | -0.00873 |
| | $\alpha_0$ (Å$^3$) | 93.985 | -0.523 | -0.181 | 0.0160 | -1.121 | 0.0 | -0.077 |
| | $\alpha_1$ (Å$^3$) | 54.018 | -0.594 | -0.534 | 0.0 | -1.767 | 0.0 | 0.0 |
| | $p_0 \times 10^2$ (eÅ) | 0.0465 | 0.0197 | 0.00956 | 0.0 | 0.0284 | 0.0 | 0.0 |
| | $P_0 \times 10^5$ (eÅ$^{-2}$) | 0.863 | 0.361 | 0.189 | 0.0 | 0.527 | 0.0 | 0.0 |

TABLE VIII. Fitting parameters for bilayer $MoS_2$/WS2.

| Stacking | Quantity | $\phi_0$ | $\phi_1^{\rm even}$ | $\phi_2^{\rm even}$ | $\phi_3^{\rm even}$ | $\phi_1^{\rm odd}$ | $\phi_2^{\rm odd}$ | $\phi_3^{\rm odd}$ |
|---|---|---|---|---|---|---|---|---|
| 3R | $\mathcal{V}_{\rm stack}$ (eV) | -0.208 | 0.0207 | -0.00403 | -0.00148 | 0.0 | 0.0 | 0.0 |
| | $d_0$ (Å) | 6.779 | 0.147 | -0.0205 | -0.00892 | -0.00215 | 0.0 | -0.00104 |
| | $\alpha_0$ (Å$^3$) | 110.162 | 1.378 | -0.188 | -0.0831 | -0.0198 | 0.0 | -0.00962 |
| | $\alpha_1$ (Å$^3$) | 63.007 | 1.872 | -0.374 | -0.117 | -0.00587 | 0.0 | -0.0351 |
| | $p_0 \times 10^2$ (eÅ) | 0.0477 | -0.0212 | 0.00397 | 0.00166 | 0.0915 | 0.0 | -0.0153 |
| | $P_0 \times 10^5$ (eÅ$^{-2}$) | 0.753 | -0.344 | 0.0707 | 0.0278 | 1.464 | 0.0 | -0.262 |
| 2H | $\mathcal{V}_{\rm stack}$ (eV) | -0.207 | -0.00556 | -0.00322 | 0.00104 | -0.0173 | 0.0 | 0.0 |
| | $d_0$ (Å) | 6.783 | -0.0521 | -0.0156 | 0.00412 | -0.121 | 0.0 | -0.00621 |
| | $\alpha_0$ (Å$^3$) | 110.27 | -0.496 | -0.144 | 0.0380 | -1.137 | 0.0 | -0.0583 |
| | $\alpha_1$ (Å$^3$) | 63.187 | -0.580 | -0.246 | 0.0490 | -1.516 | 0.0 | -0.0890 |
| | $p_0 \times 10^2$ (eÅ) | 0.0495 | 0.0111 | 0.00319 | 0.0 | 0.0175 | 0.0 | 0.00150 |
| | $P_0 \times 10^5$ (eÅ$^{-2}$) | 0.777 | 0.177 | 0.0570 | -0.121 | 0.283 | 0.0 | 0.0251 |

TABLE IX. Fitting parameters for bilayer $MoSe_2$/WSe2.

| Stacking | Quantity | $\phi_0$ | $\phi_1^{\text{even}}$ | $\phi_2^{\text{even}}$ | $\phi_3^{\text{even}}$ | $\phi_1^{\text{odd}}$ | $\phi_2^{\text{odd}}$ | $\phi_3^{\text{odd}}$ |
|---|---|---|---|---|---|---|---|---|
| 3R | $\mathcal{V}_{\text{stack}}$ (eV) | -0.117 | 0.0225 | -0.00436 | -0.00151 | -0.00190 | 0.0 | 0.0 |
| | $d_0$ (Å) | 6.560 | 0.150 | -0.0210 | -0.00781 | -0.00628 | 0.0 | 0.0 |
| | $\alpha_0$ (Å$^3$) | 100.542 | 1.279 | -0.168 | -0.0654 | -0.0555 | 0.0 | 0.00658 |
| | $\alpha_1$ (Å$^3$) | 55.141 | 2.332 | -0.453 | -0.185 | -0.0420 | 0.0 | 0.0141 |
| | $p_0 \times 10^2$ (eÅ) | 0.0902 | -0.130 | 0.0249 | 0.00728 | 0.112 | 0.0 | -0.0191 |
| | $P_0 \times 10^5$ (eÅ$^{-2}$) | 15.207 | -2.508 | 0.523 | 0.1487 | 1.953 | 0.0 | -0.357 |
| 2H | $\mathcal{V}_{\text{stack}}$ (eV) | -0.115 | -0.00607 | -0.00354 | 0.00128 | -0.0188 | 0.0 | 0.0 |
| | $d_0$ (Å) | 6.566 | -0.0526 | -0.0178 | 0.00460 | -0.125 | 0.0 | -0.00614 |
| | $\alpha_0$ (Å$^3$) | 100.643 | -0.449 | -0.147 | 0.0361 | -1.062 | 0.0 | -0.0476 |
| | $\alpha_1$ (Å$^3$) | 55.268 | -0.835 | -0.390 | 0.107 | -1.935 | 0.0 | -0.163 |
| | $p_0 \times 10^2$ (eÅ) | 0.898 | 0.0543 | 0.0219 | -0.00455 | 0.109 | 0.0 | 0.00932 |
| | $P_0 \times 10^5$ (eÅ$^{-2}$) | 15.101 | 1.011 | 0.450 | -0.0960 | 2.110 | 0.0 | 0.159 |

TABLE X. Fitting parameters for bilayer $MoS_2$/WSe2.

| Stacking | Quantity | $\phi_0$ | $\phi_1^{\text{even}}$ | $\phi_2^{\text{even}}$ | $\phi_3^{\text{even}}$ | $\phi_1^{\text{odd}}$ | $\phi_2^{\text{odd}}$ | $\phi_3^{\text{odd}}$ |
|---|---|---|---|---|---|---|---|---|
| 3R | $\mathcal{V}_{\text{stack}}$ (eV) | -0.142 | 0.0225 | -0.00439 | -0.00153 | 0.00133 | 0.0 | 0.0 |
| | $d_0$ (Å) | 6.565 | 0.149 | -0.210 | -0.00819 | 0.00656 | 0.0 | 0.0 |
| | $\alpha_0$ (Å$^3$) | 103.777 | 1.328 | -0.181 | -0.0722 | 0.0625 | 0.0 | -0.00873 |
| | $\alpha_1$ (Å$^3$) | 58.021 | 2.019 | -0.411 | -0.118 | 0.0260 | 0.0 | -0.0104 |
| | $p_0 \times 10^2$ (eÅ) | -0.771 | 0.0736 | -0.0107 | -0.00354 | 0.109 | 0.0 | -0.0194 |
| | $P_0 \times 10^5$ (eÅ$^{-2}$) | -12.979 | 1.515 | -0.255 | -0.0816 | 1.905 | 0.0 | -0.362 |
| 2H | $\mathcal{V}_{\text{stack}}$ (eV) | -0.140 | -0.00655 | -0.00354 | 0.00121 | -0.0184 | 0.0 | 0.0 |
| | $d_0$ (Å) | 6.598 | -0.0538 | -0.0185 | 0.00440 | -0.123 | 0.0 | -0.00652 |
| | $\alpha_0$ (Å$^3$) | 103.858 | -0.484 | -0.162 | 0.0391 | -1.010 | 0.0 | -0.0577 |
| | $\alpha_1$ (Å$^3$) | 58.184 | -0.667 | -0.303 | 0.0640 | -1.589 | 0.0 | -0.0907 |
| | $p_0 \times 10^2$ (eÅ) | -0.769 | -0.0255 | -0.00723 | 0.00169 | -0.0580 | 0.0 | -0.00353 |
| | $P_0 \times 10^5$ (eÅ$^{-2}$) | -12.916 | -0.520 | -0.181 | 0.0430 | -1.210 | 0.0 | -0.0757 |

TABLE XI. Fitting parameters for bilayer $MoSe_2$/WS2.

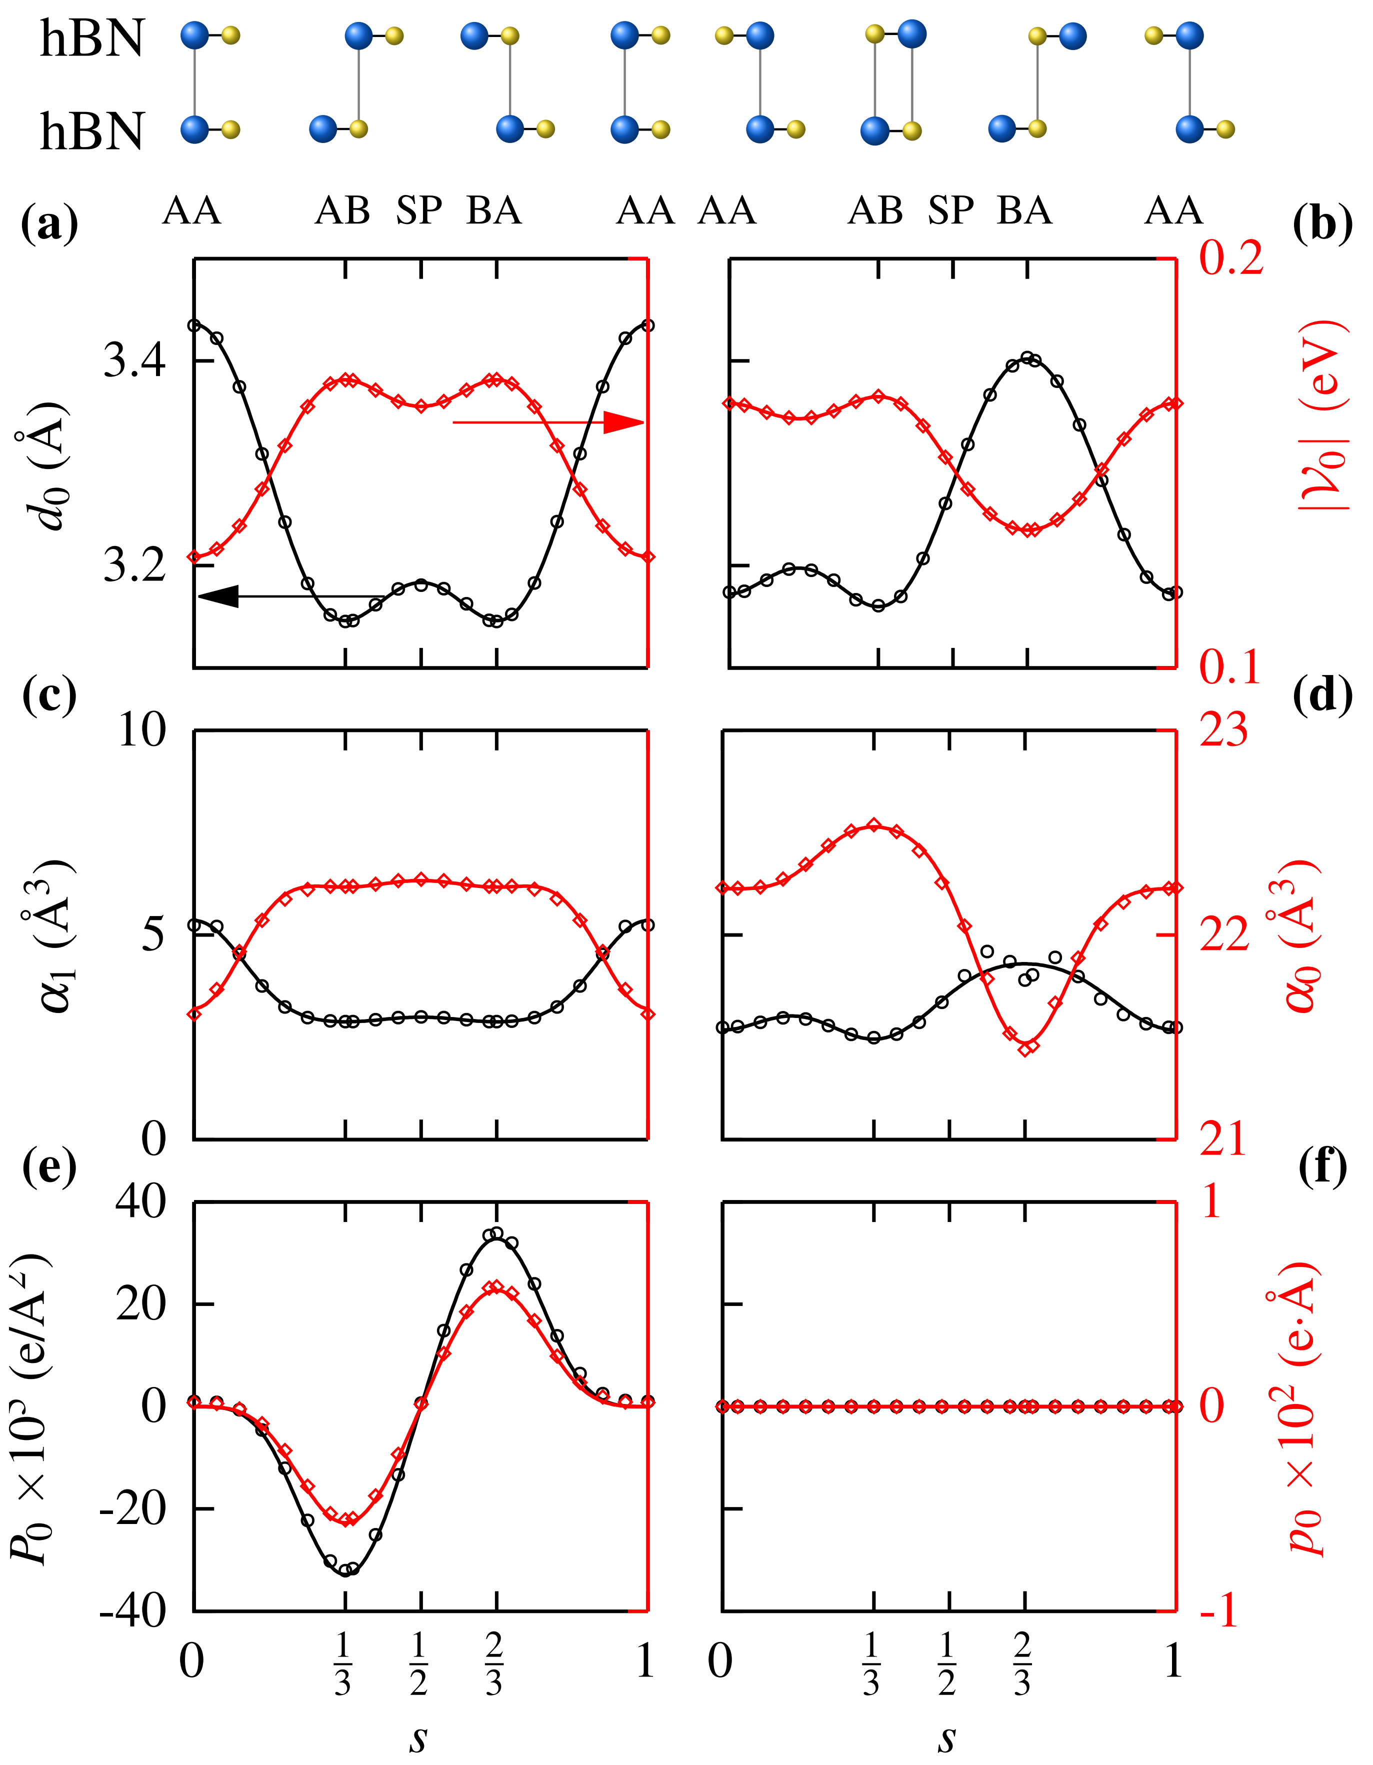


FIG. 1. Results from first-principles calculations (hollow points) and fitting (solid curves) for bilayer hBN.

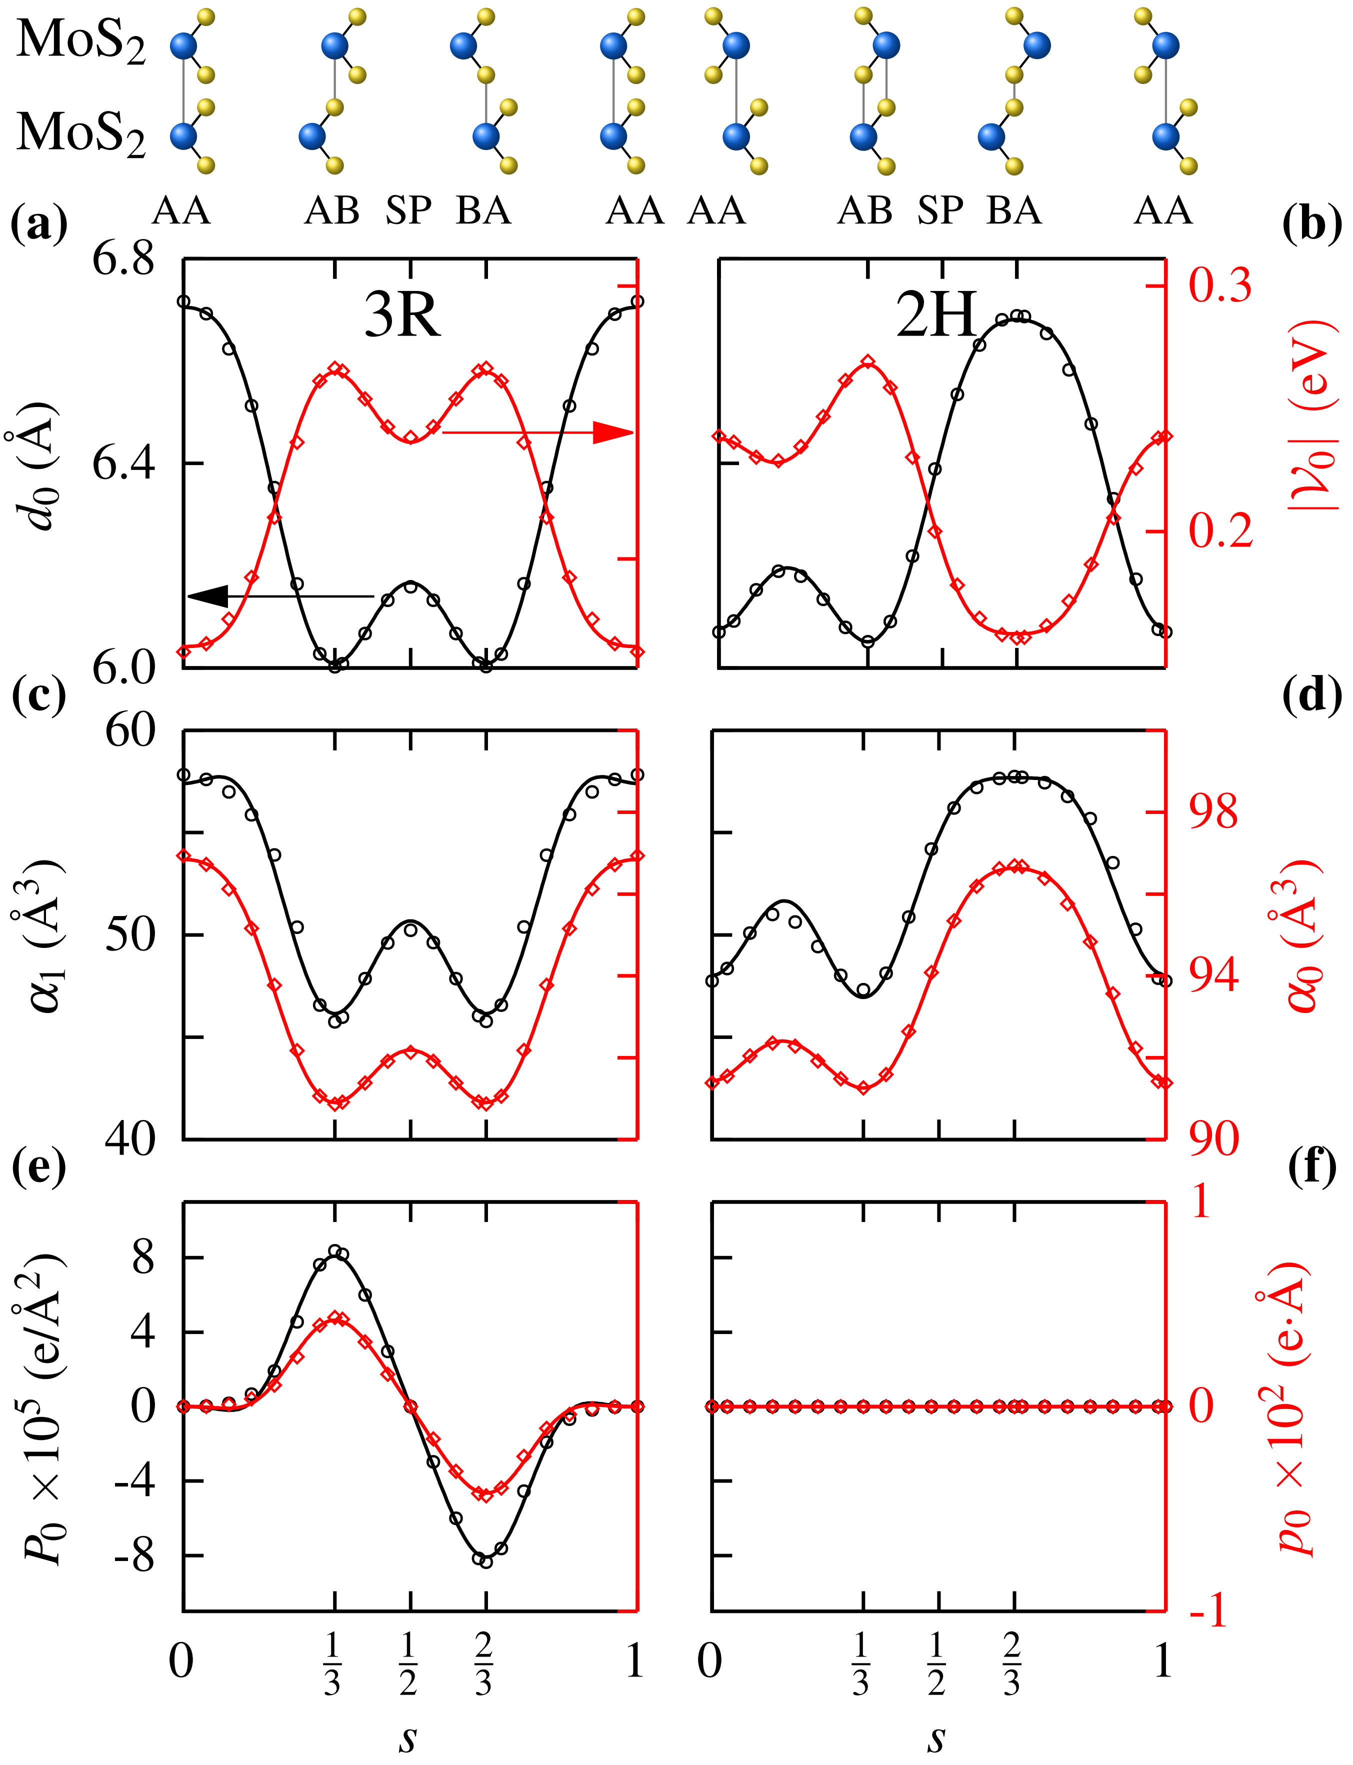


FIG. 2. Results from first-principles calculations (hollow points) and fitting (solid curves) for bilayer $MoS_2$.

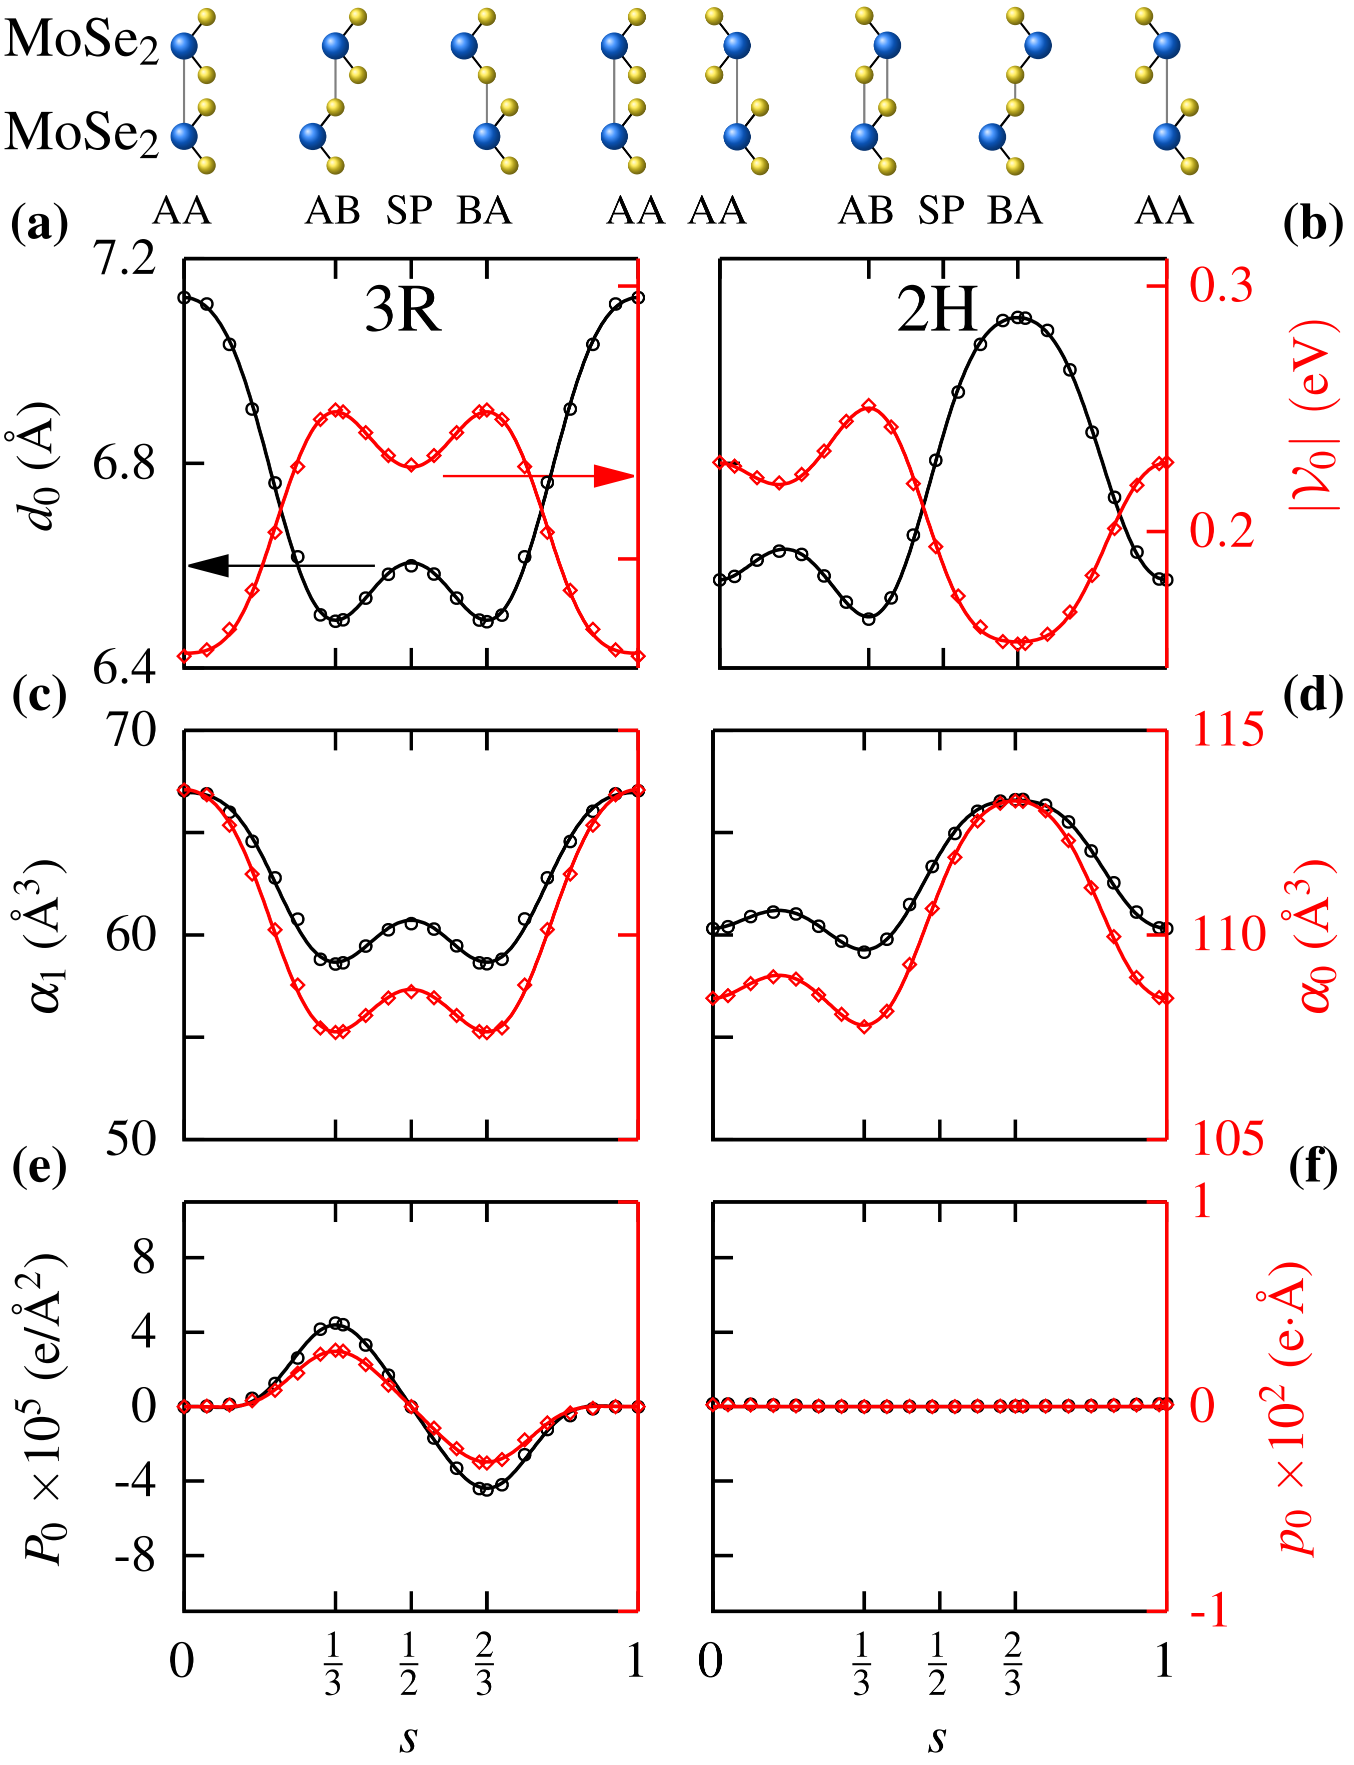


FIG. 3. Results from first-principles calculations (hollow points) and fitting (solid curves) for bilayer $MoSe_2$

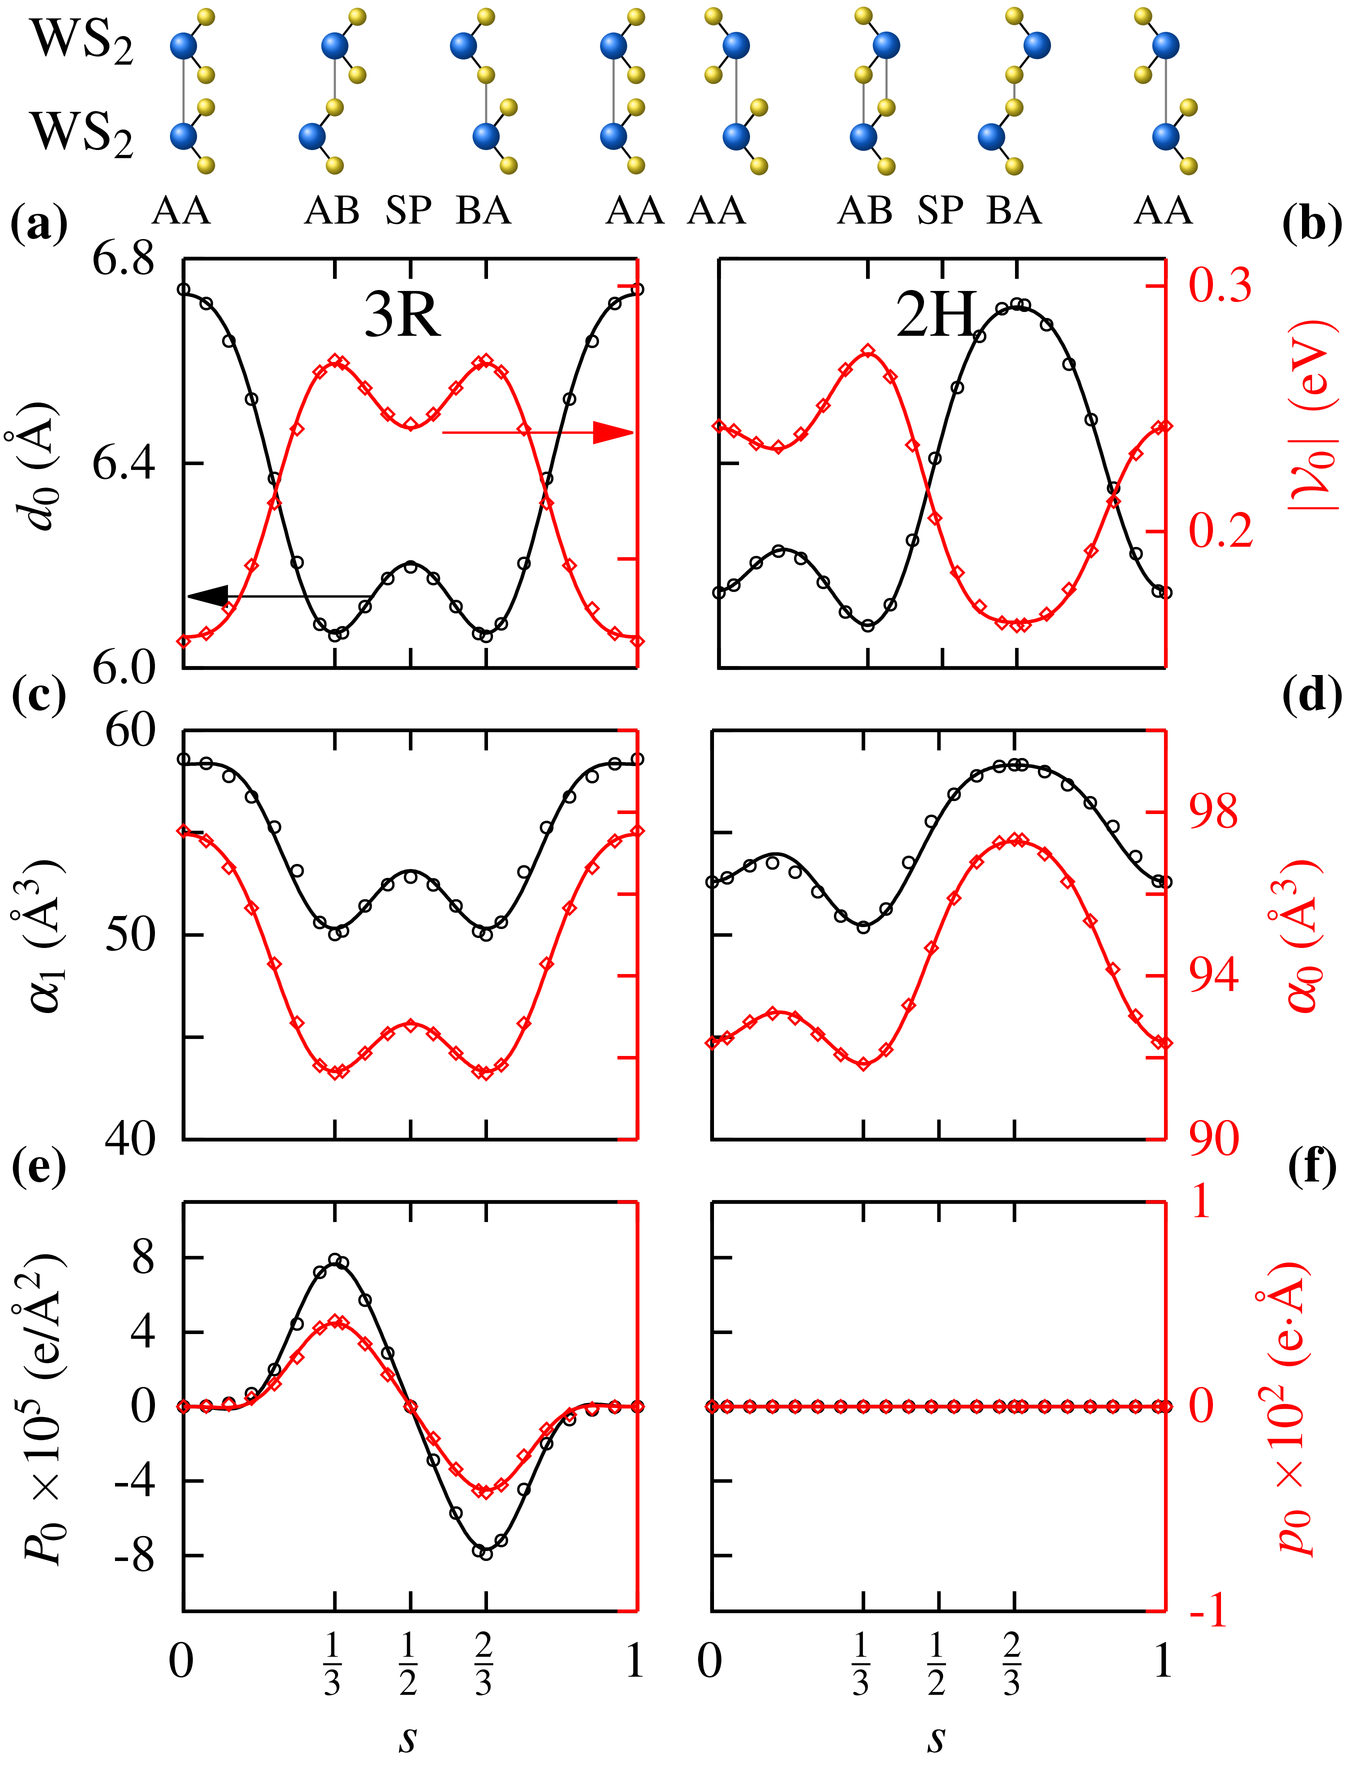


FIG. 4. Results from first-principles calculations (hollow points) and fitting (solid curves) for bilayer $WS_2$

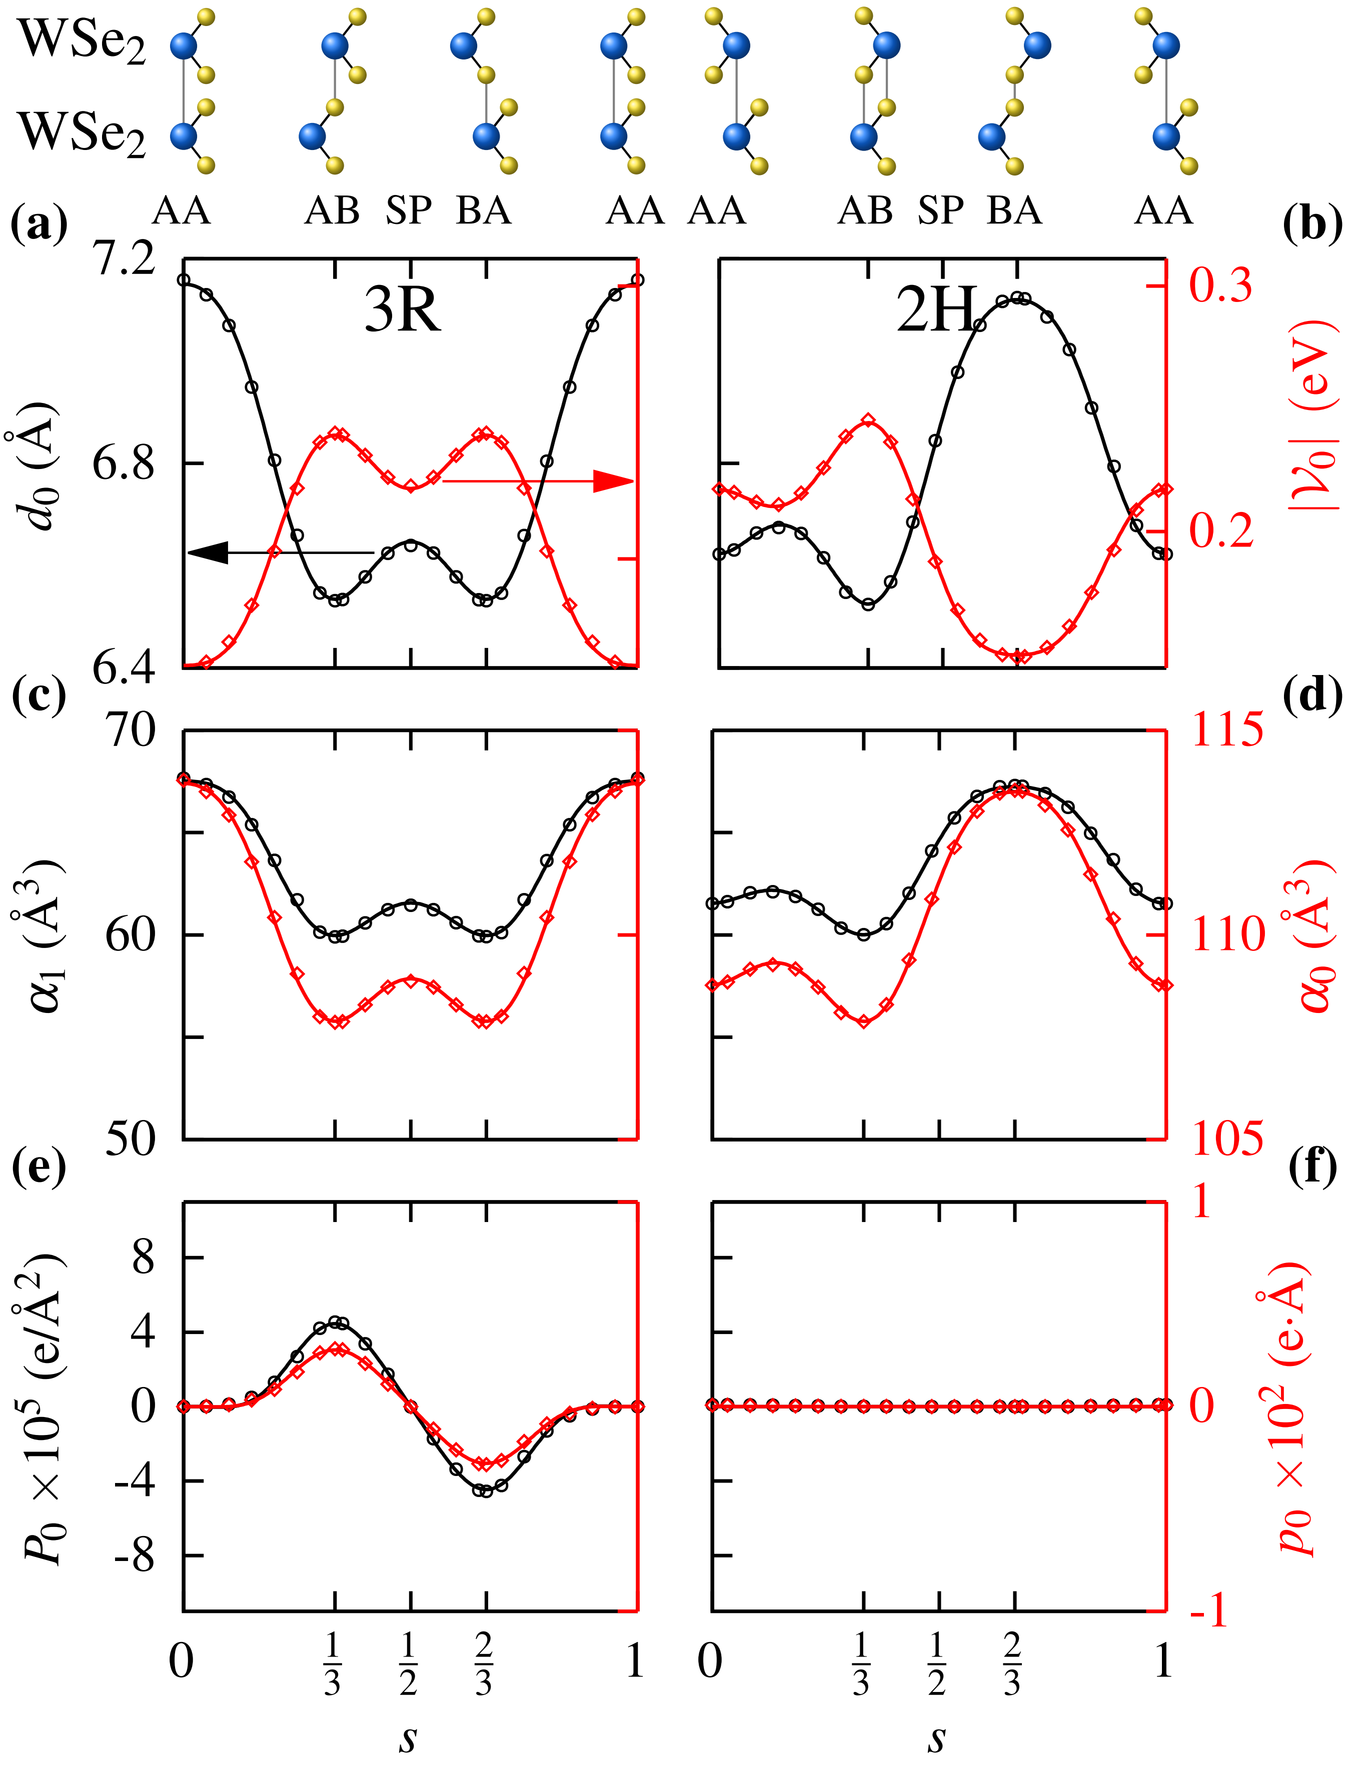


FIG. 5. Results from first-principles calculations (hollow points) and fitting (solid curves) for bilayer $WSe_2$

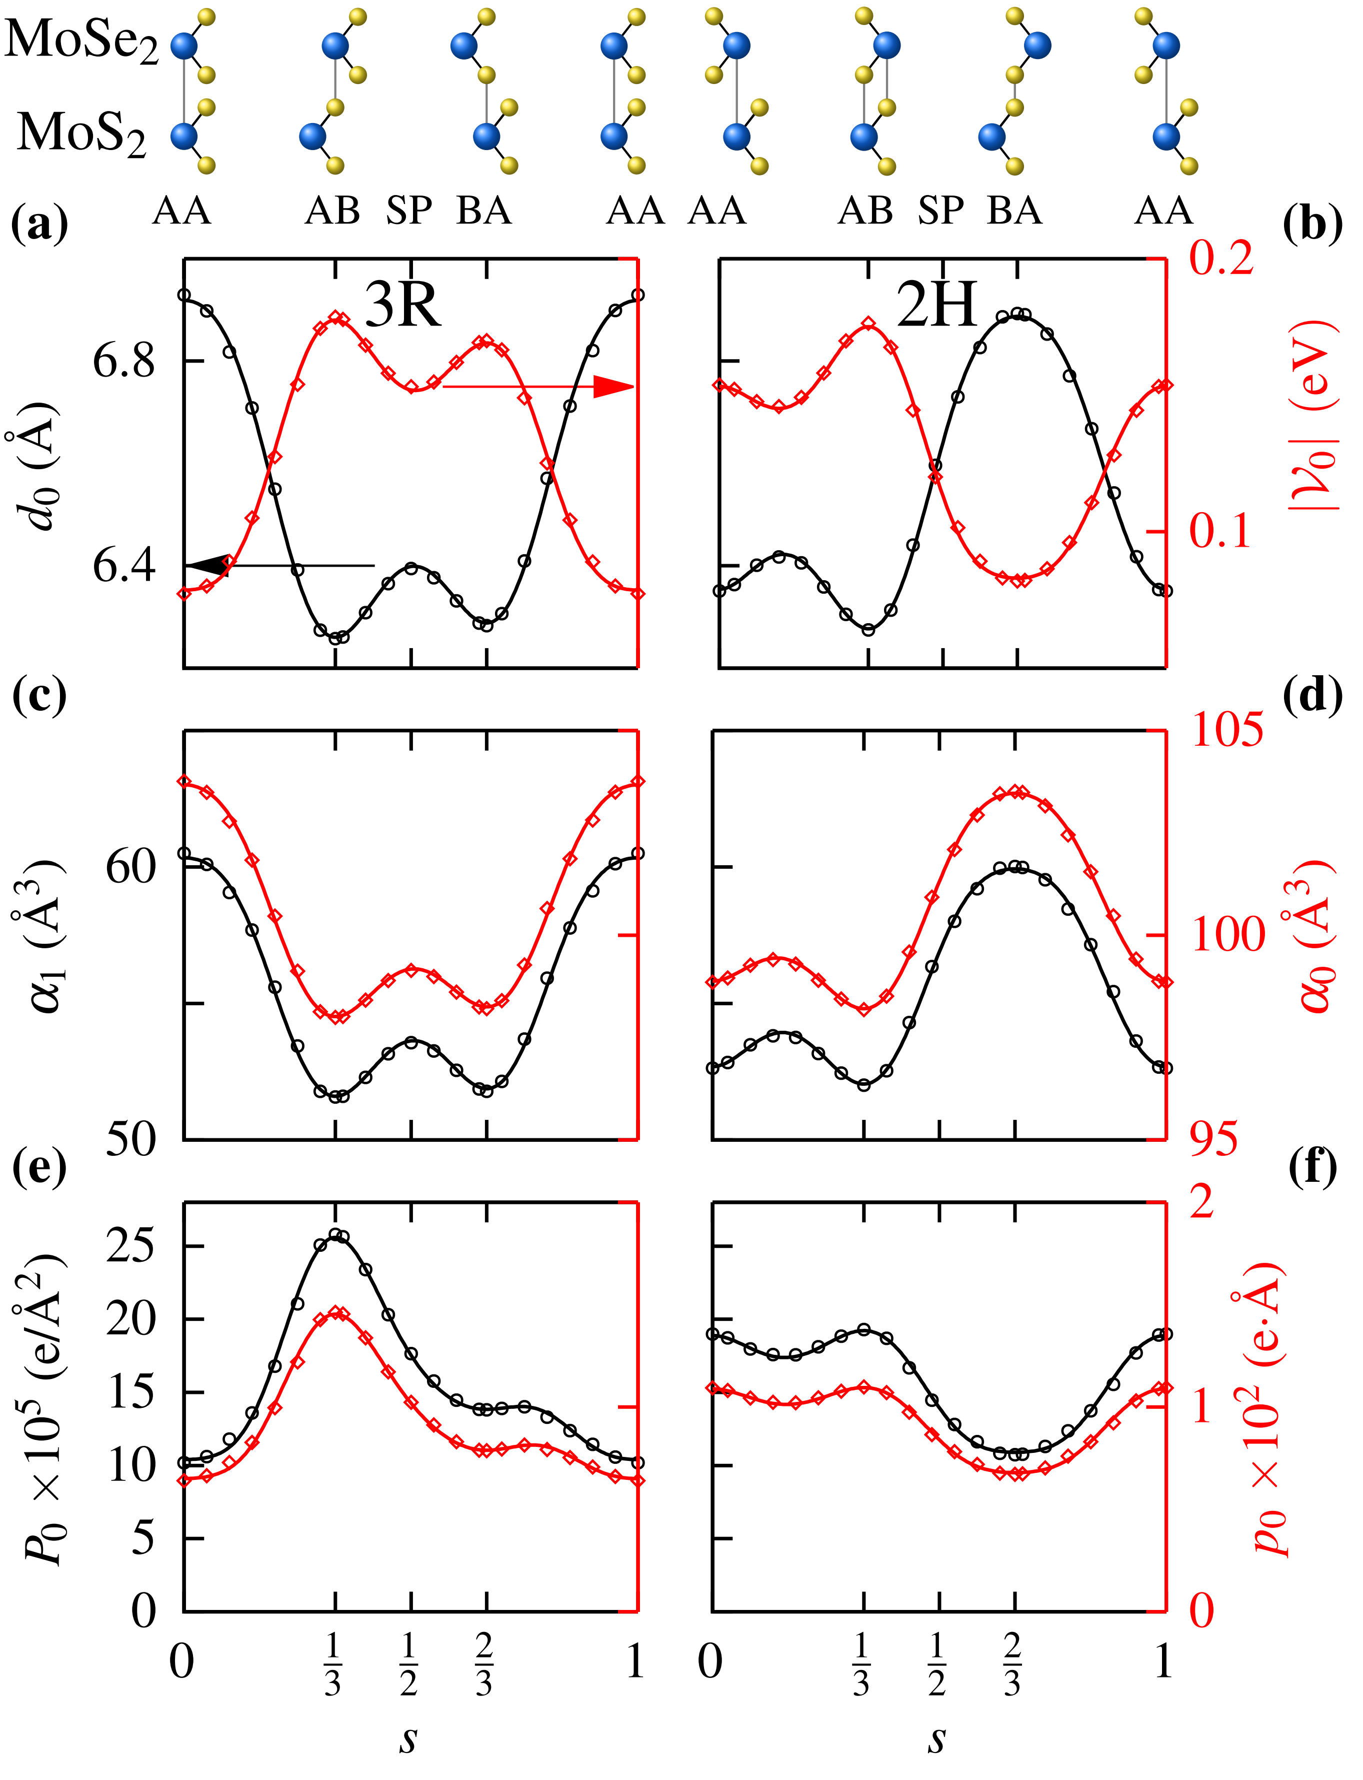


FIG. 6. Results from first-principles calculations (hollow points) and fitting (solid curves) for bilayer $MoS_2$/MoSe2

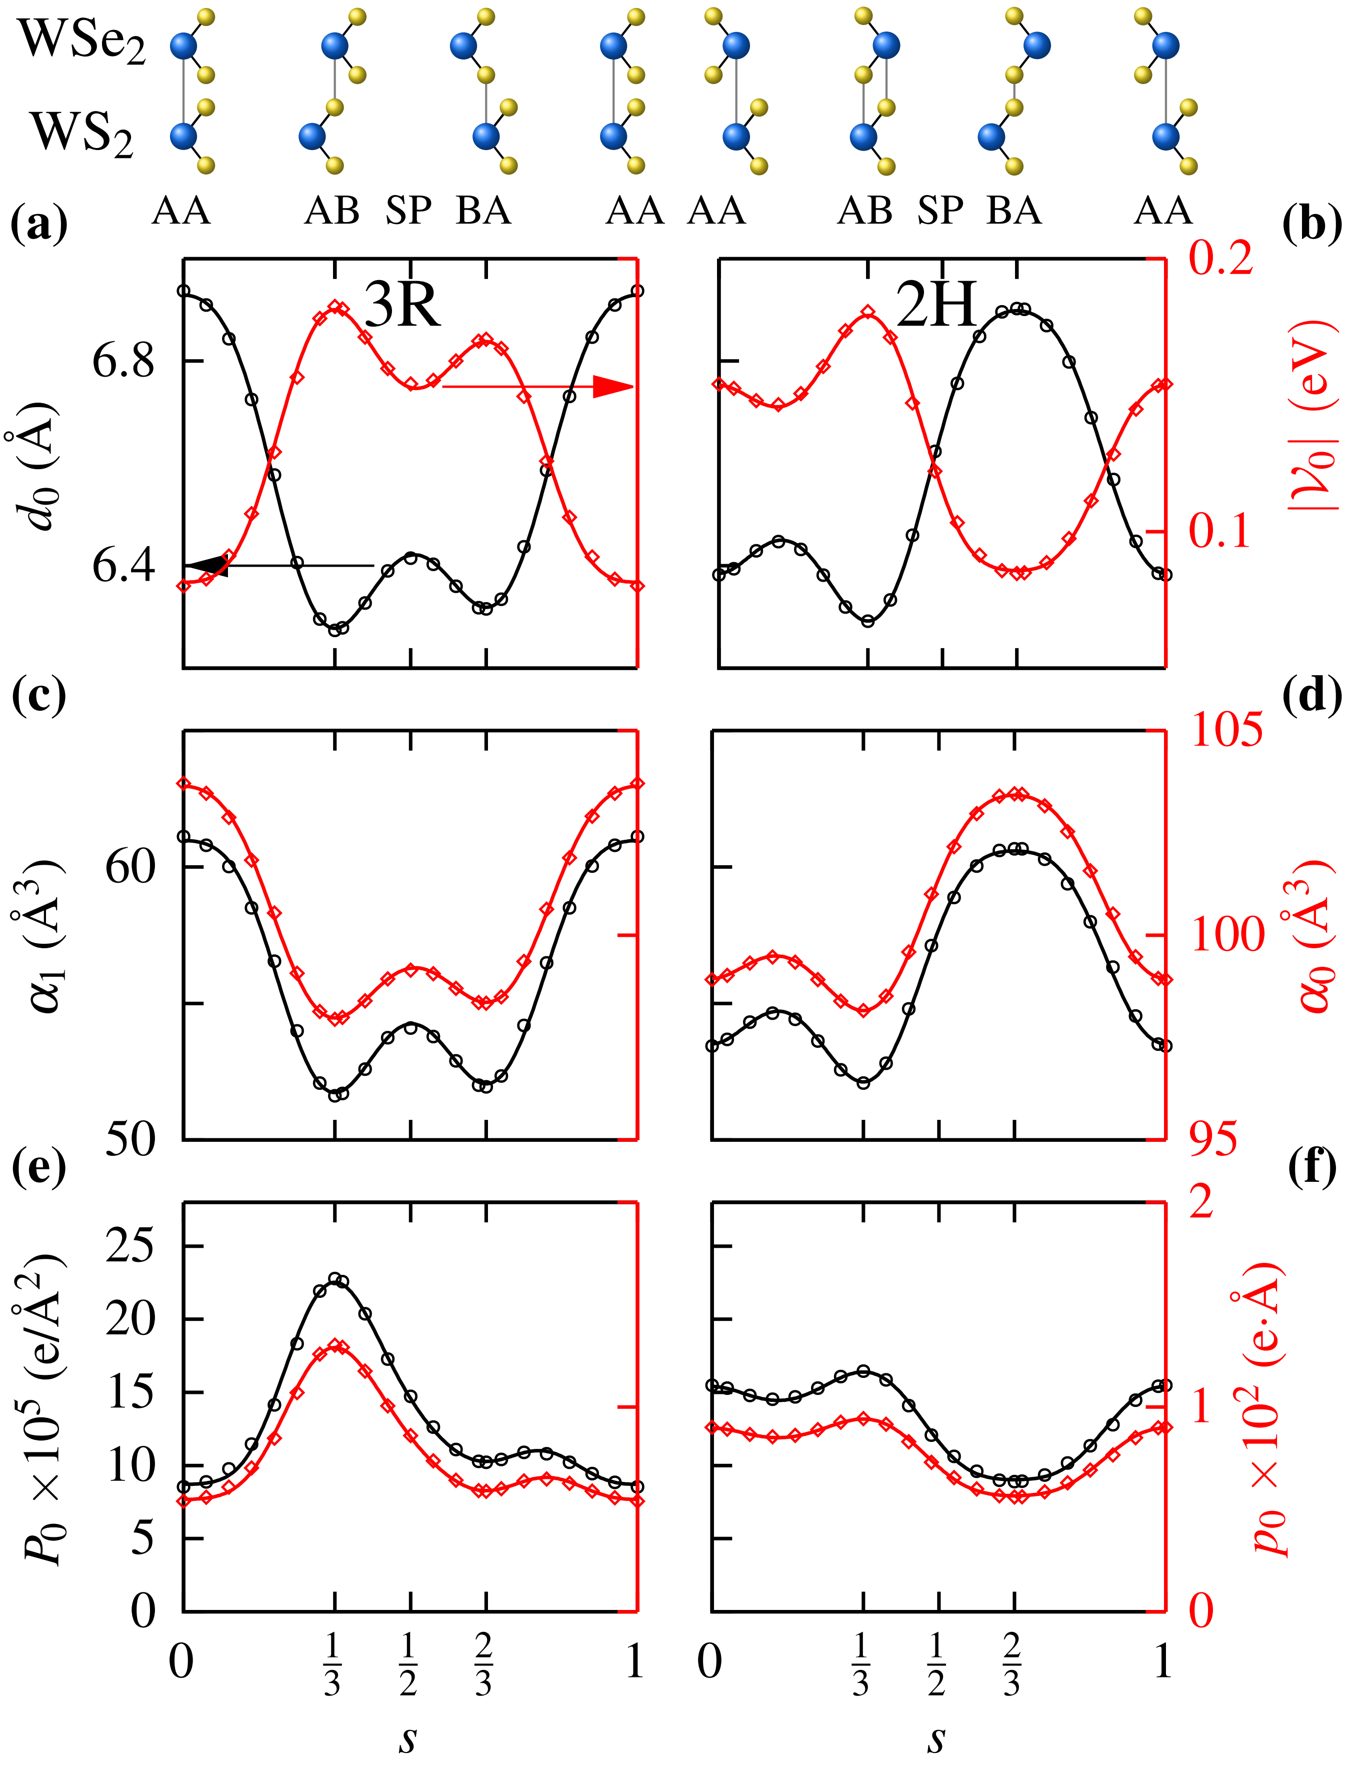


FIG. 7. Results from first-principles calculations (hollow points) and fitting (solid curves) for bilayer $WS_2$/WSe2

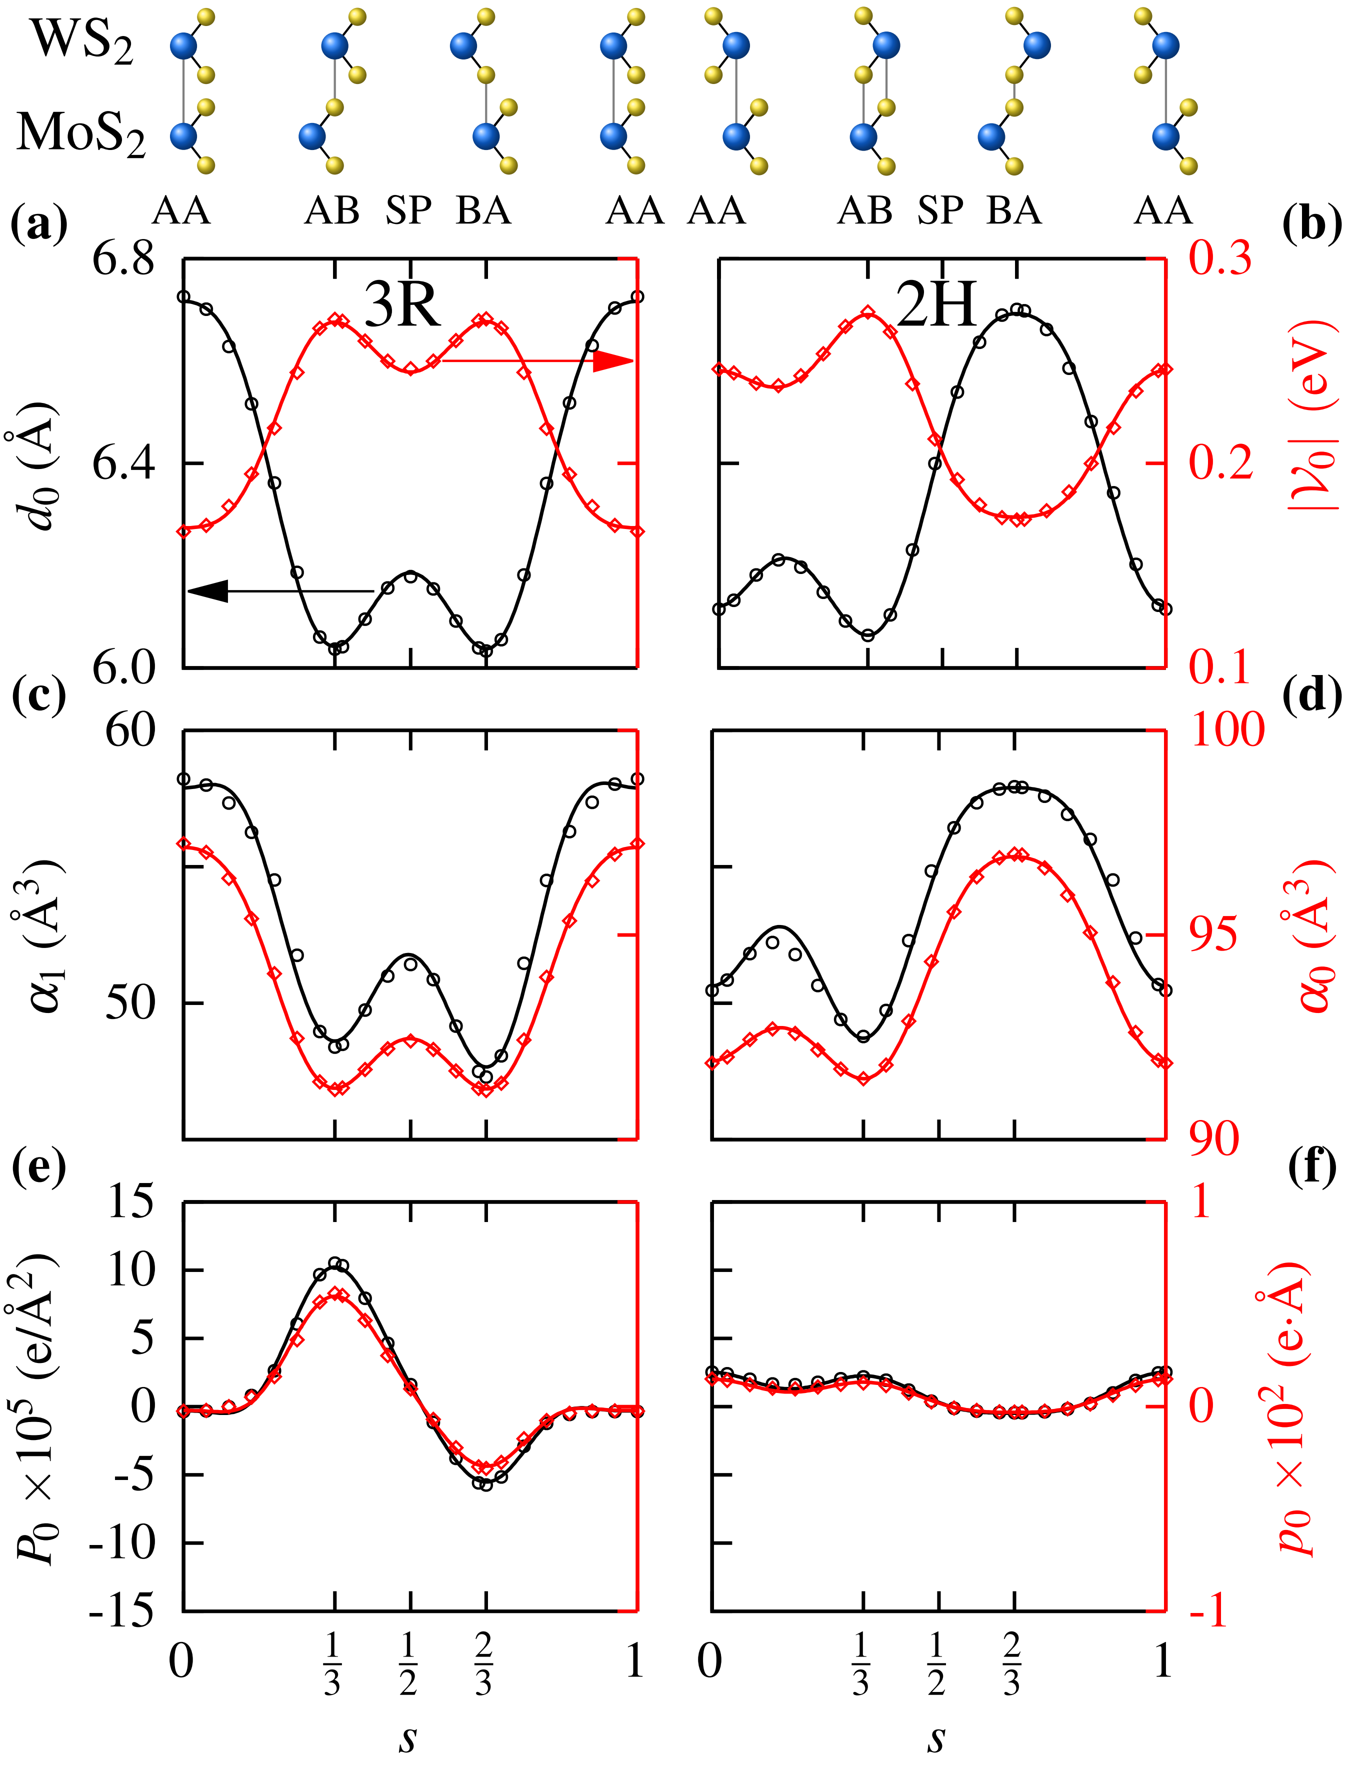


FIG. 8. Results from first-principles calculations (hollow points) and fitting (solid curves) for bilayer $MoS_2$/WS2

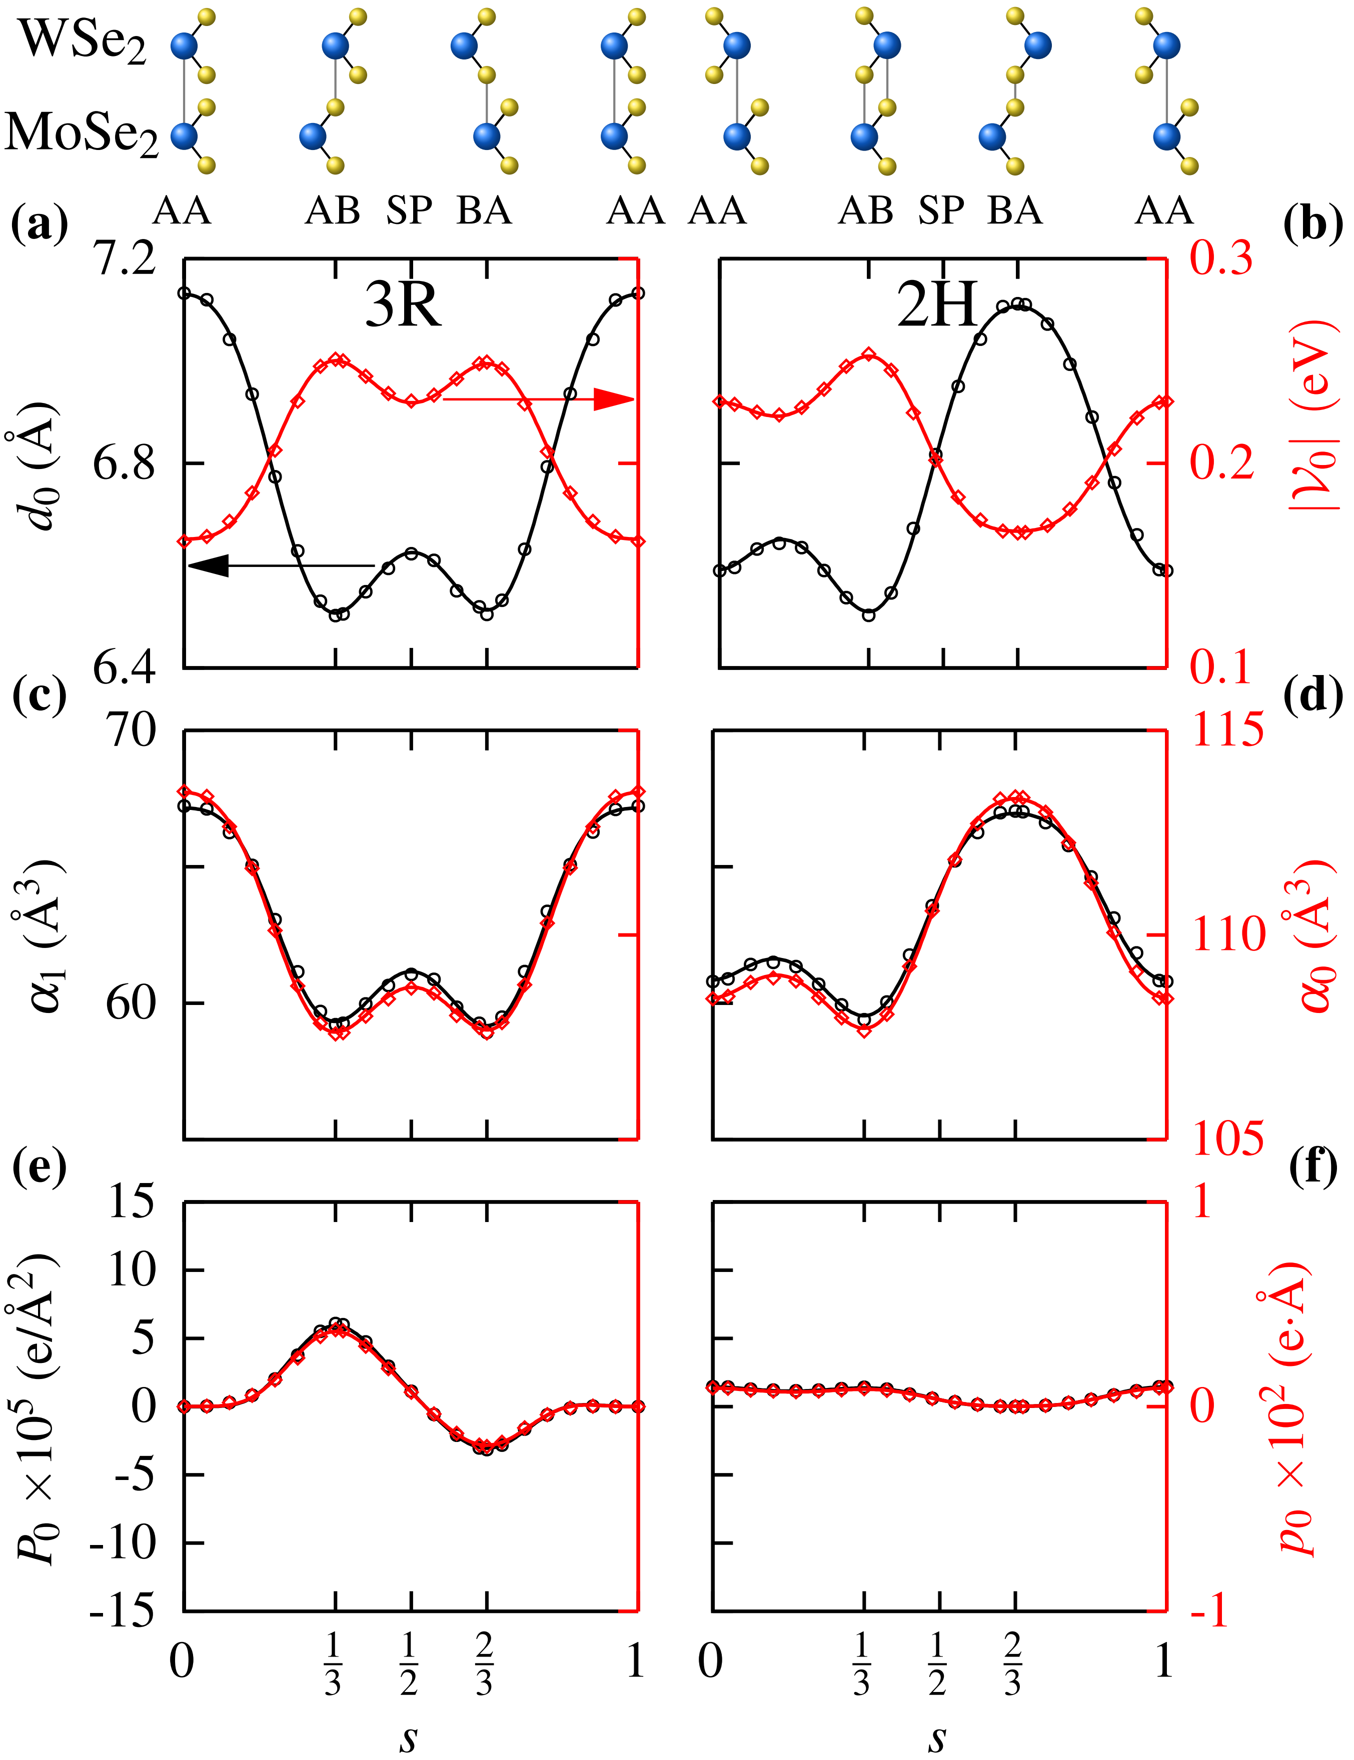


FIG. 9. Results from first-principles calculations (hollow points) and fitting (solid curves) for bilayer $MoSe_2$/WSe2

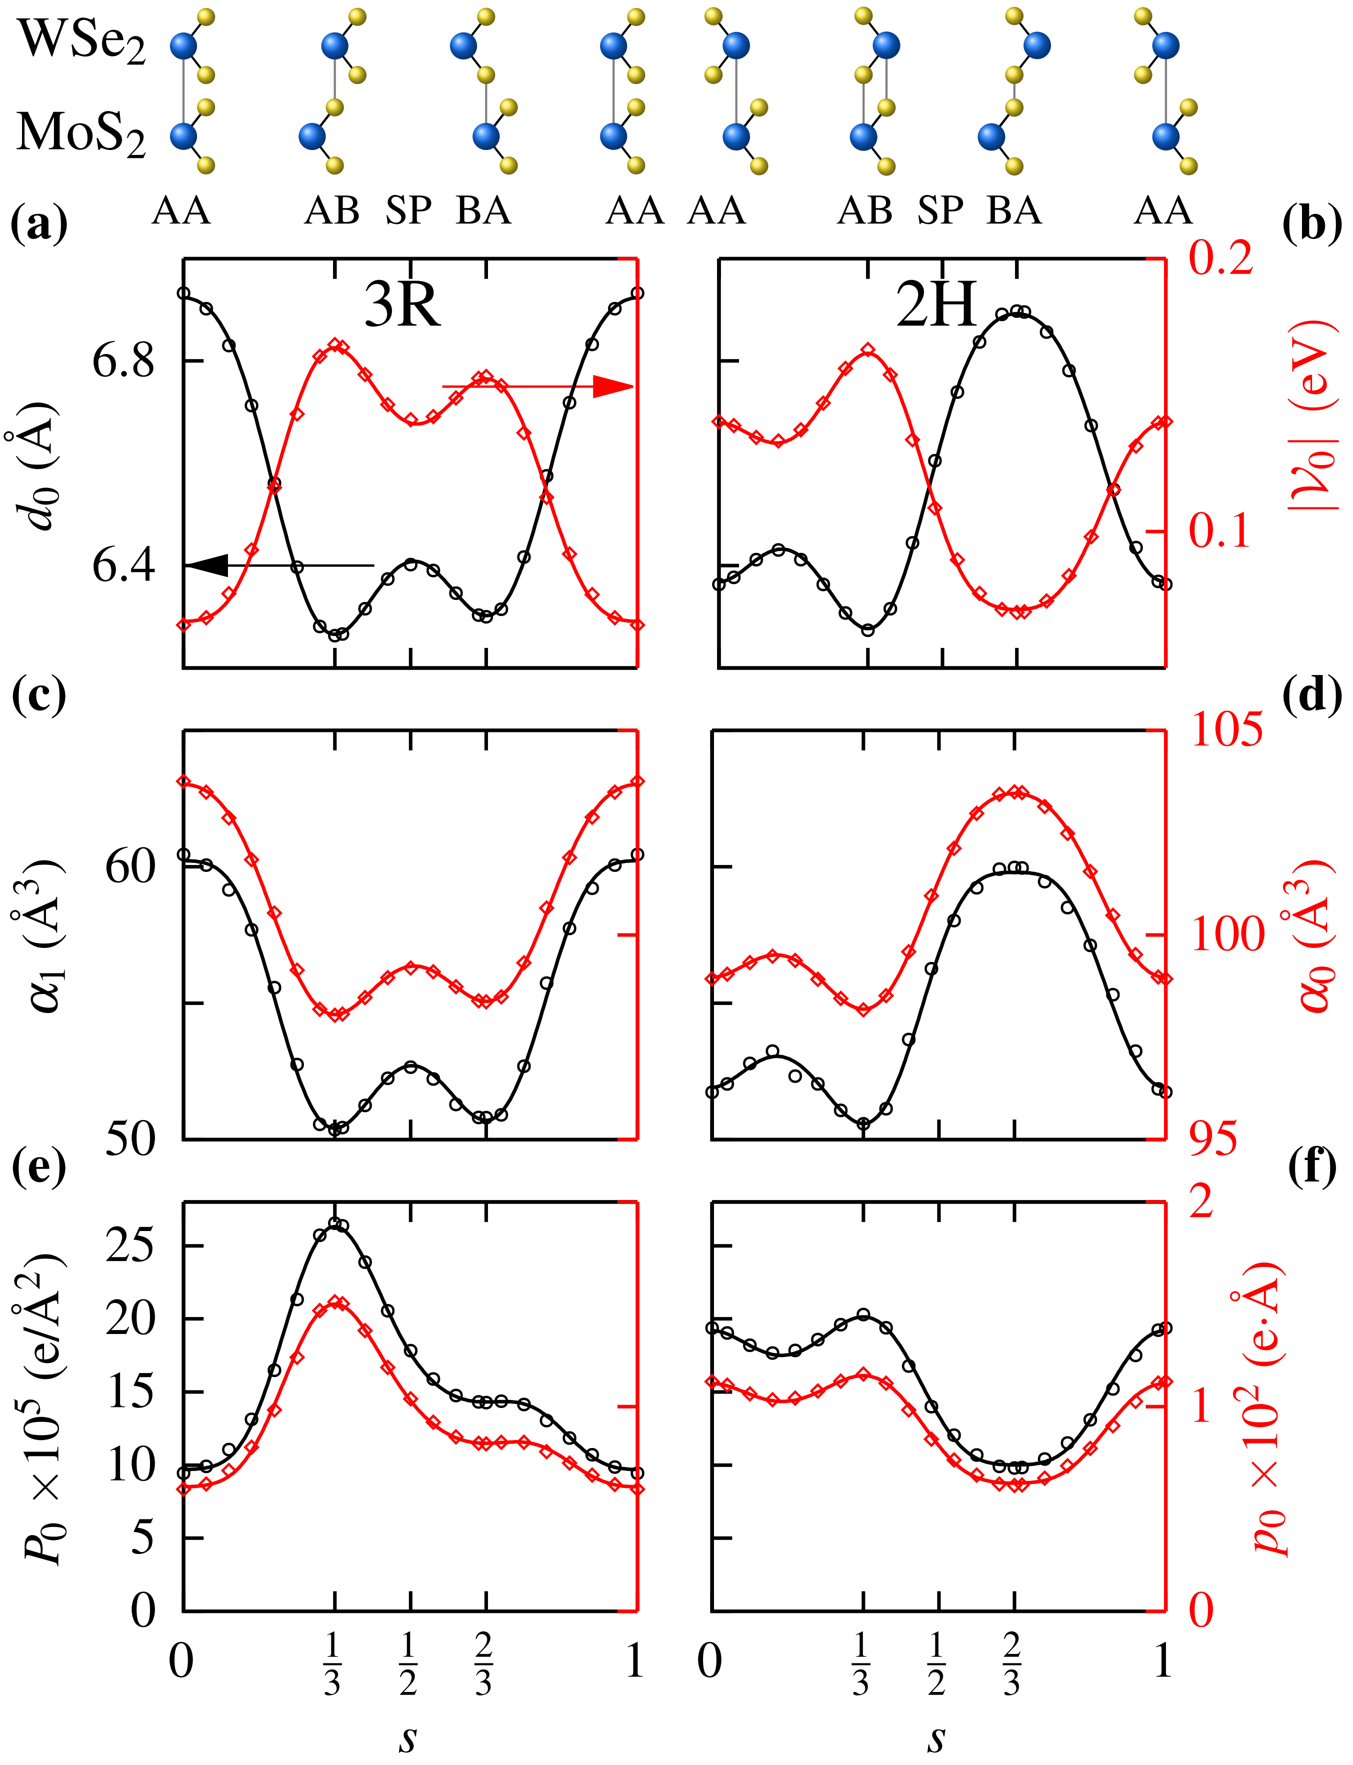


FIG. 10. Results from first-principles calculations (hollow points) and fitting (solid curves) for bilayer $MoS_2$/WSe2

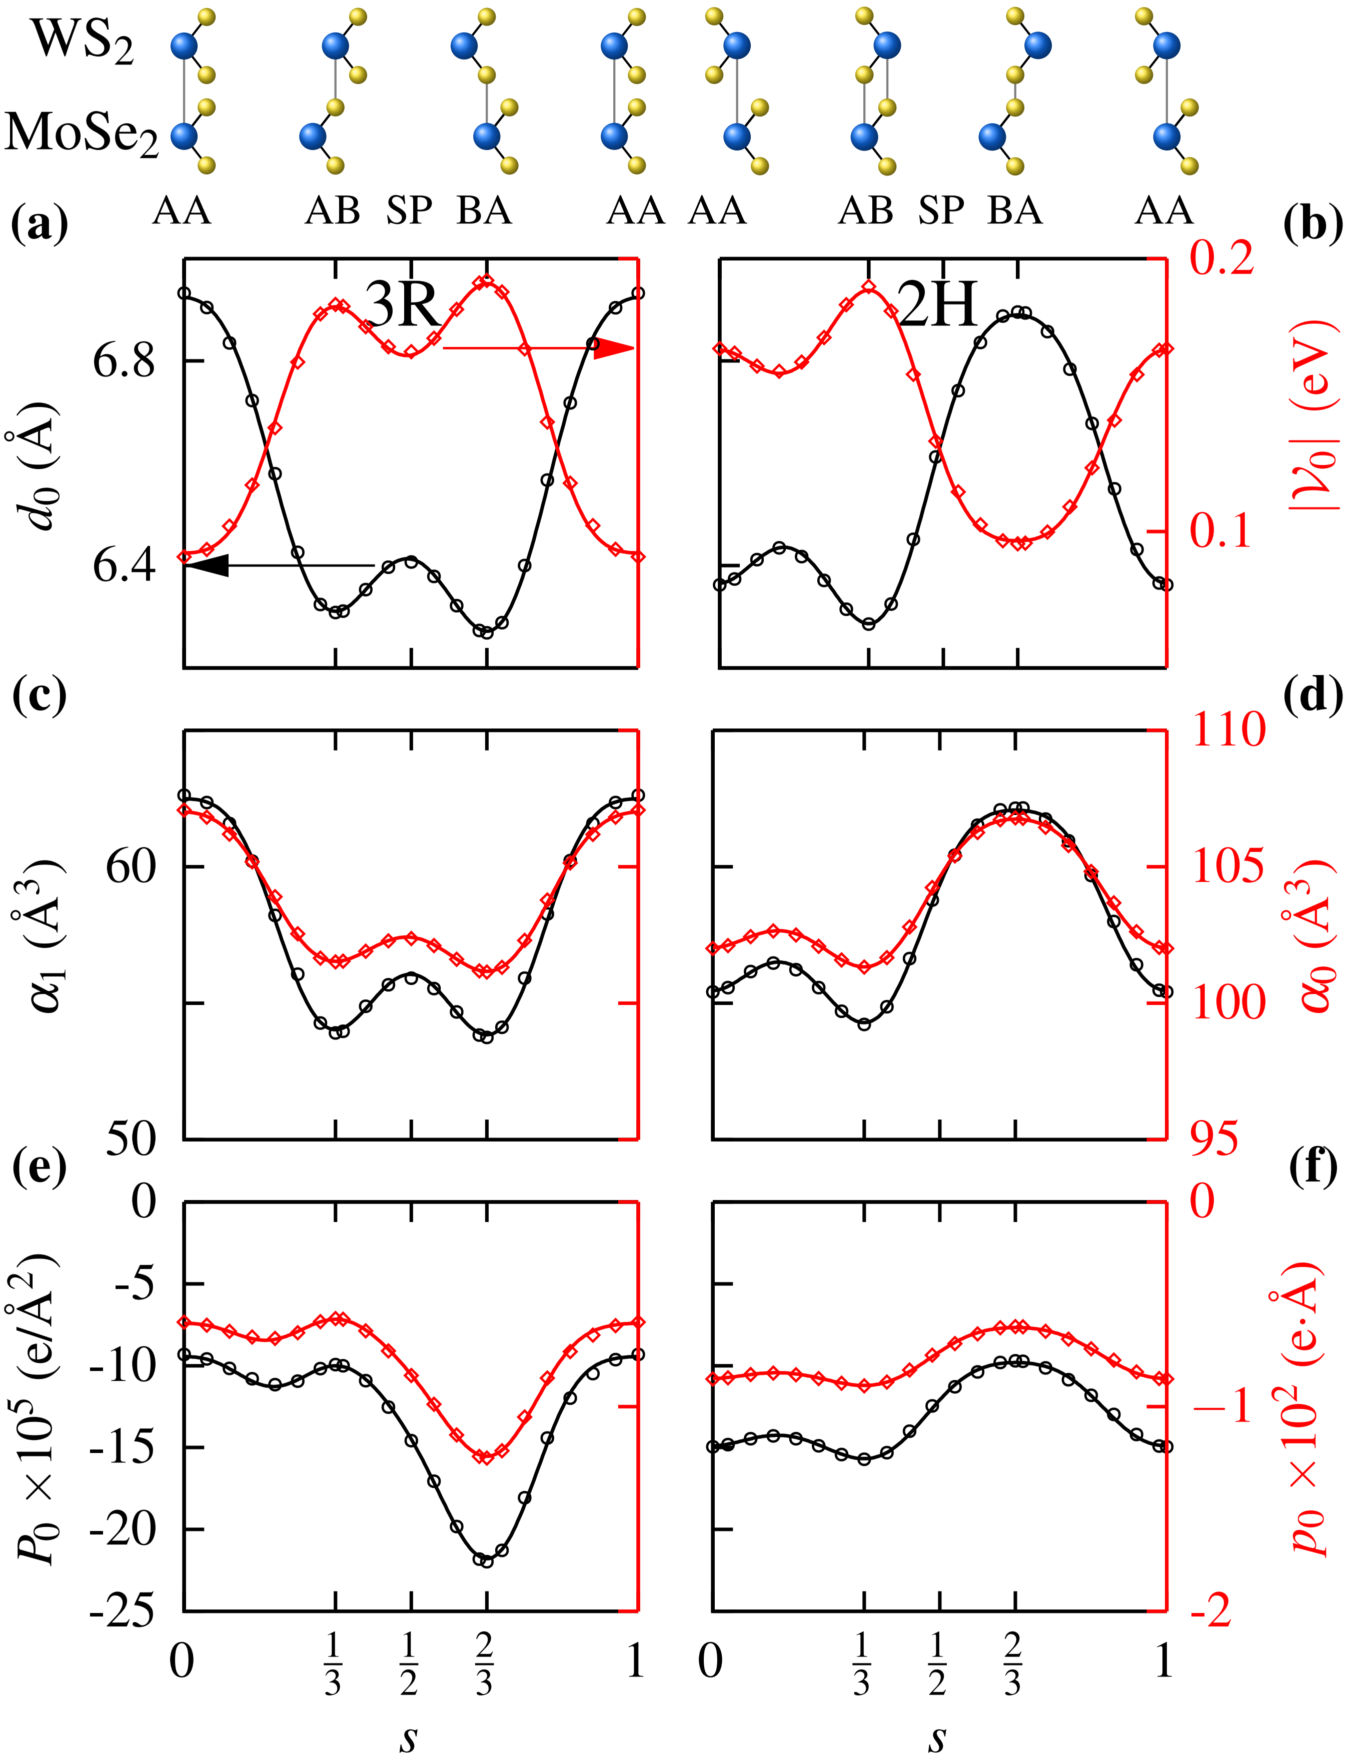


FIG. 11. Results from first-principles calculations (hollow points) and fitting (solid curves) for bilayer $MoSe_2$/WS2

## II. ADDITIONAL DATA ON TWIST ANGLE AND ELECTRIC FIELD DEPENDENCE OF STACKING DOMAINS

### 3R stacking

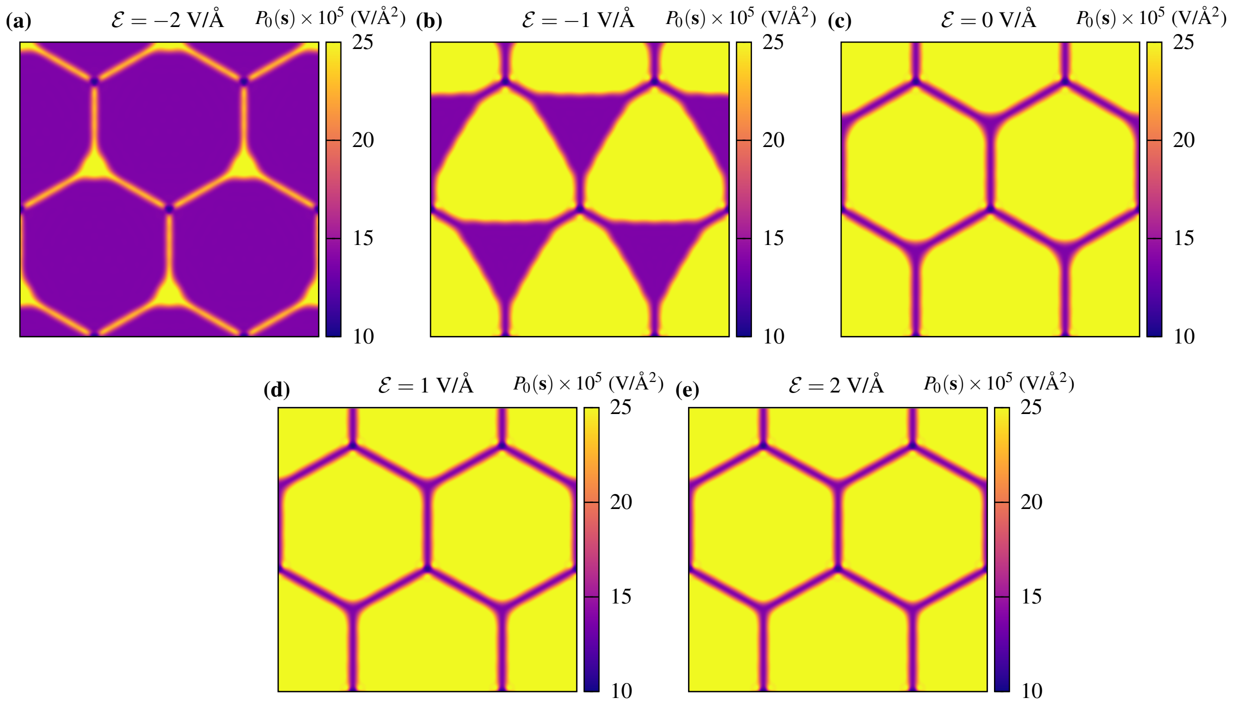


FIG. 12. Lattice relaxtion for 3R-stacked bilayer $MoS_2/MoSe_2$ at a twist angle of $\theta = 0.1^\circ$ for several electric field values.

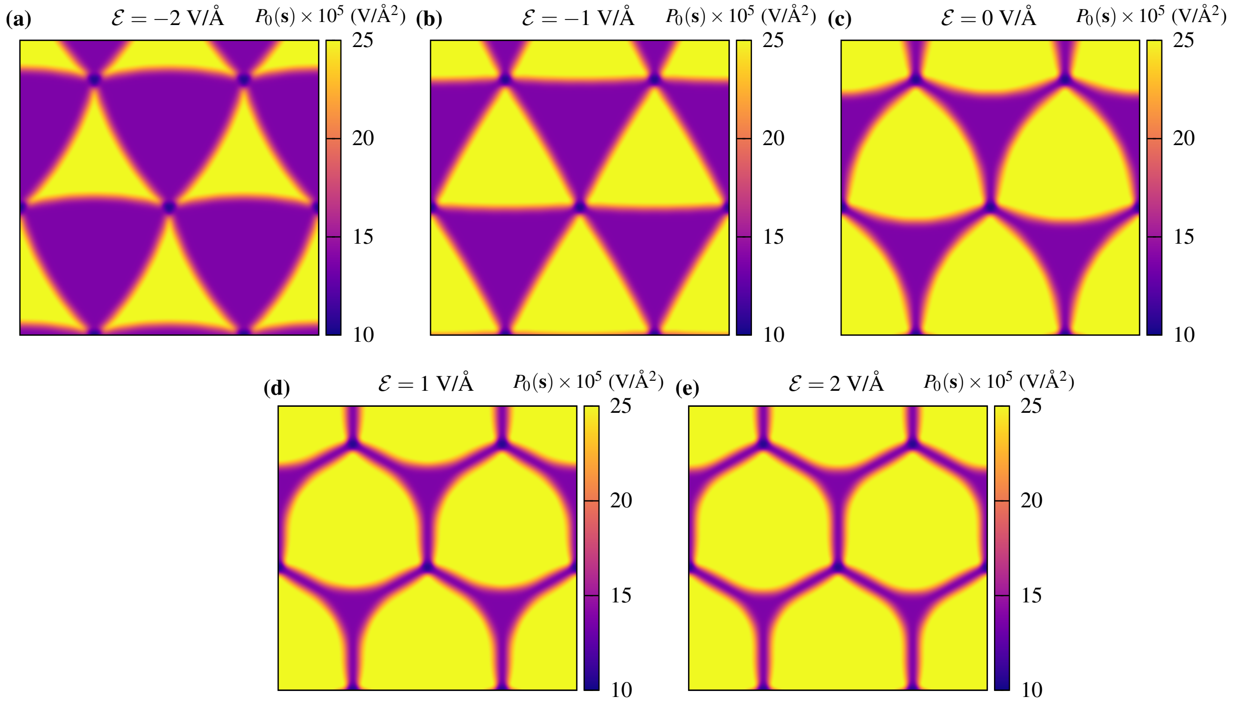


FIG. 13. Lattice relaxtion for 3R-stacked bilayer $MoS_2/MoSe_2$ at a twist angle of $\theta = 0.3^\circ$ for several electric field values.

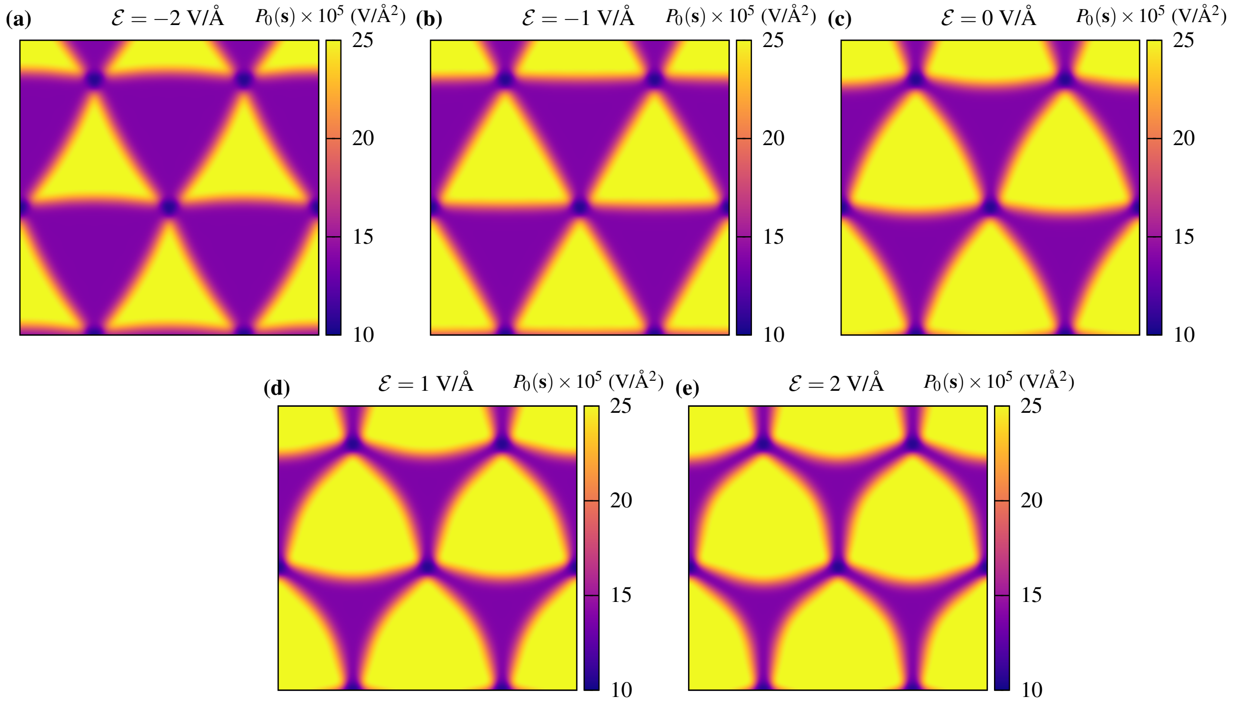


FIG. 14. Lattice relaxtion for 3R-stacked bilayer $MoS_2/MoSe_2$ at a twist angle of $\theta = 0.5^\circ$ for several electric field values.

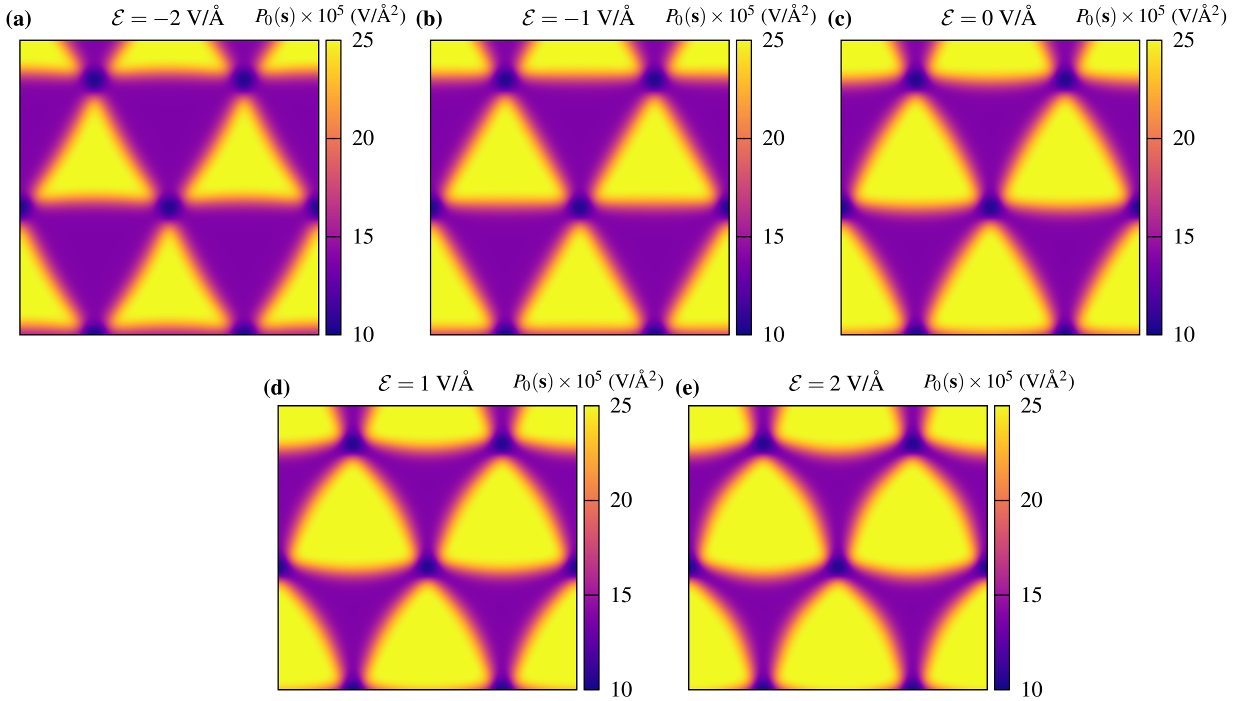


FIG. 15. Lattice relaxtion for 3R-stacked bilayer $MoS_2/MoSe_2$ at a twist angle of $\theta = 0.7^\circ$ for several electric field values.

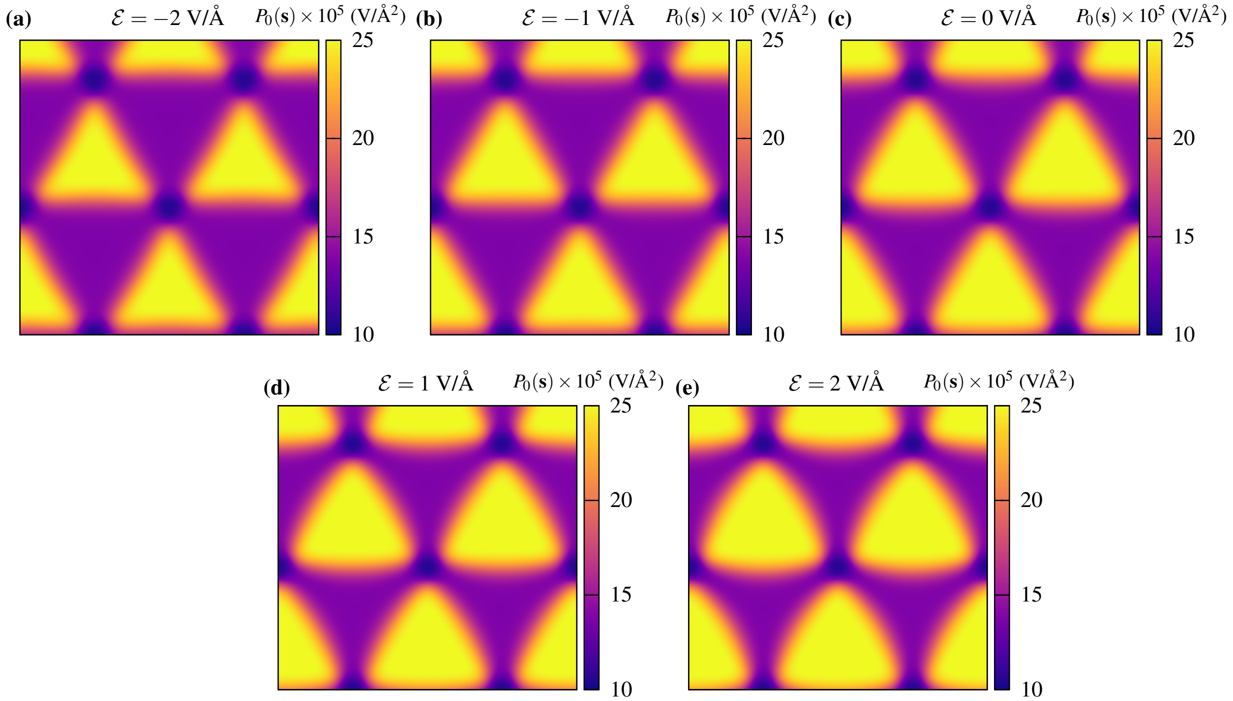


FIG. 16. Lattice relaxtion for 3R-stacked bilayer $MoS_2/MoSe_2$ at a twist angle of $\theta = 0.9^\circ$ for several electric field values.

**2H stacking**

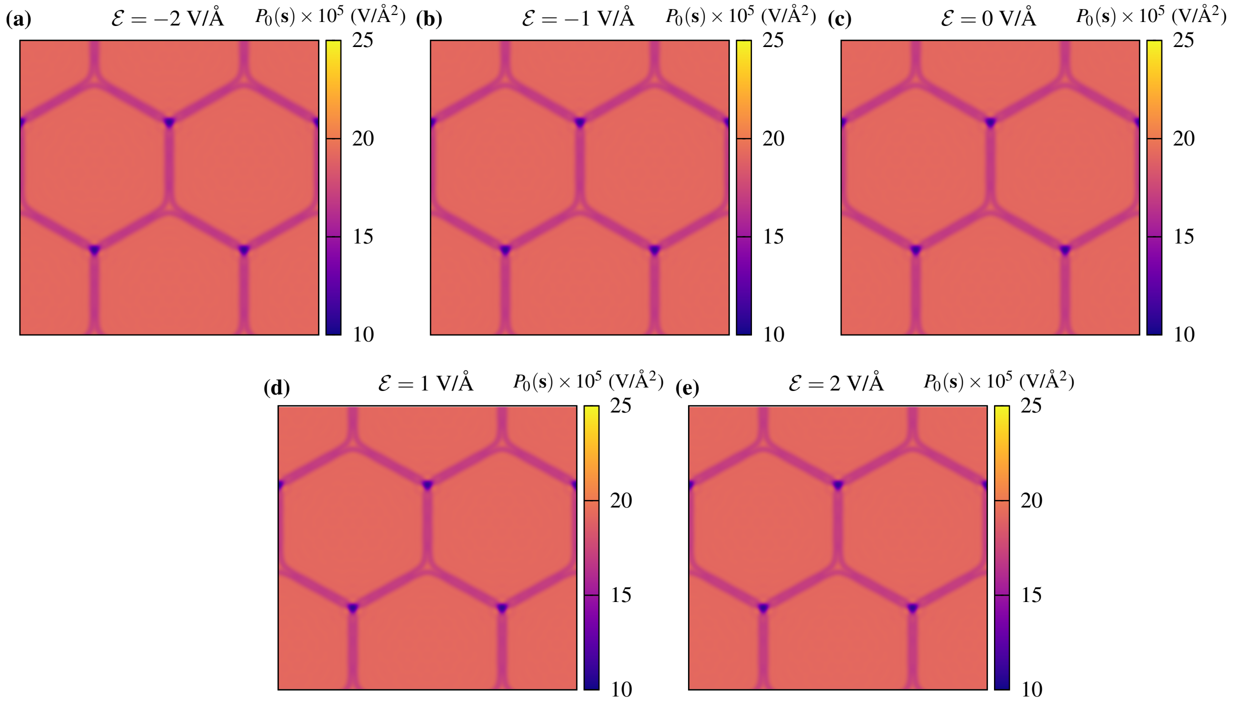


FIG. 17. Lattice relaxtion for 2H-stacked bilayer $MoS_2/MoSe_2$ at a twist angle of $\theta = 0.1^\circ$ for several electric field values.

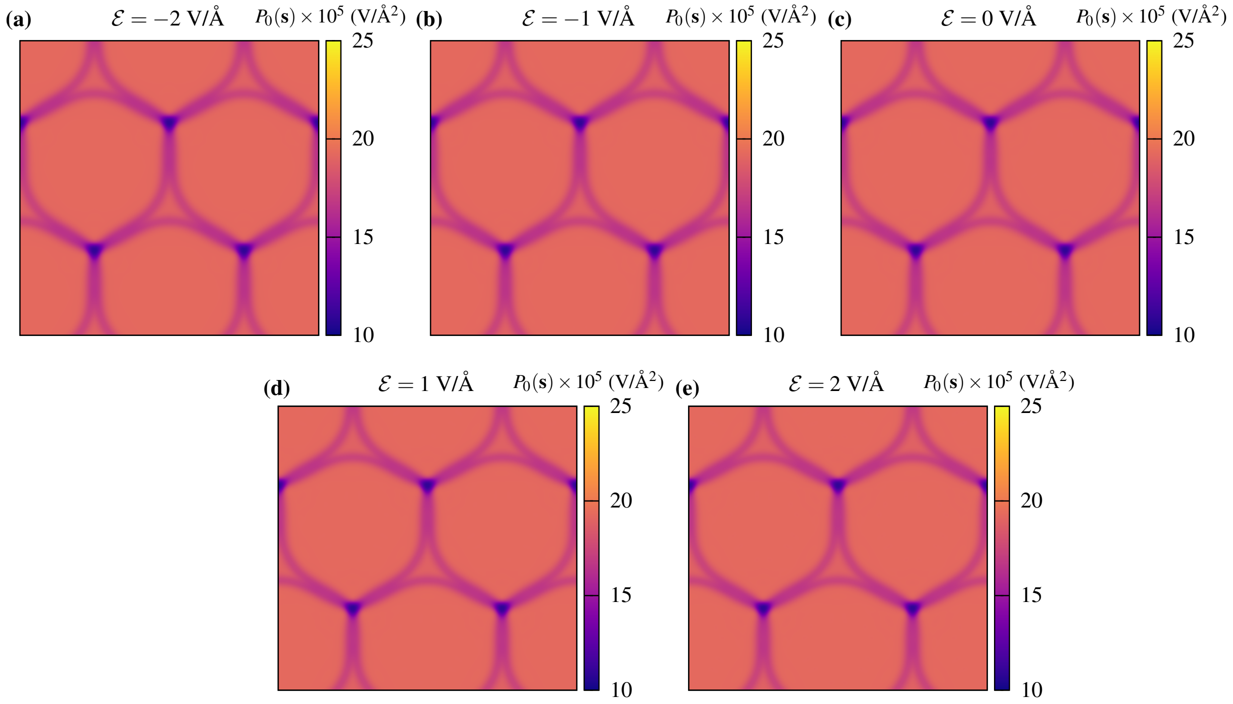


FIG. 18. Lattice relaxtion for 2H-stacked bilayer $MoS_2/MoSe_2$ at a twist angle of $\theta = 0.3^\circ$ for several electric field values.

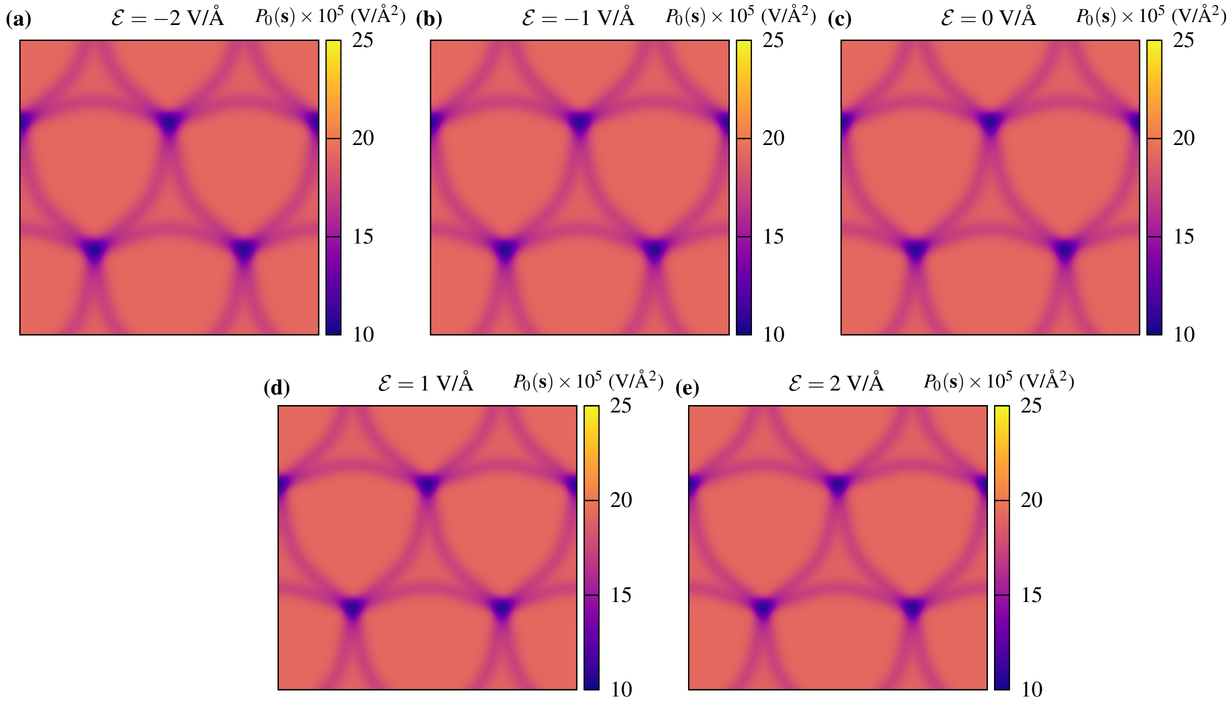


FIG. 19. Lattice relaxtion for 2H-stacked bilayer $MoS_2/MoSe_2$ at a twist angle of $\theta = 0.5^\circ$ for several electric field values.

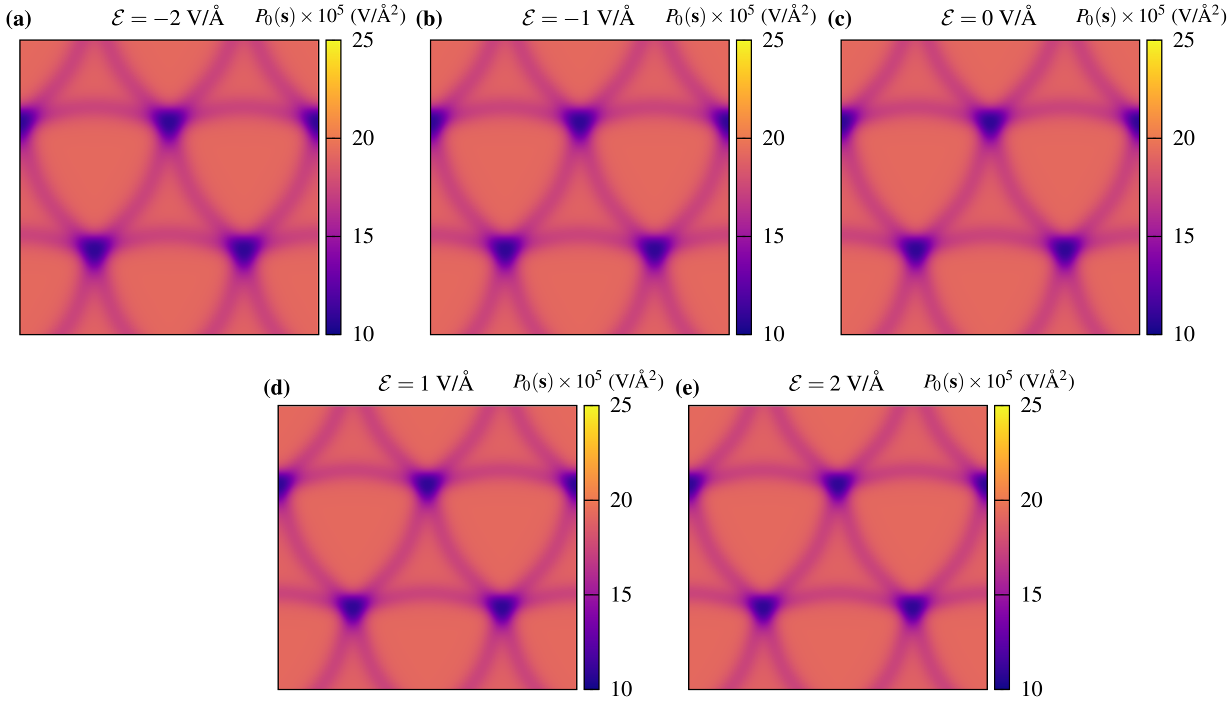


FIG. 20. Lattice relaxtion for 2H-stacked bilayer $MoS_2/MoSe_2$ at a twist angle of $\theta = 0.7^\circ$ for several electric field values.

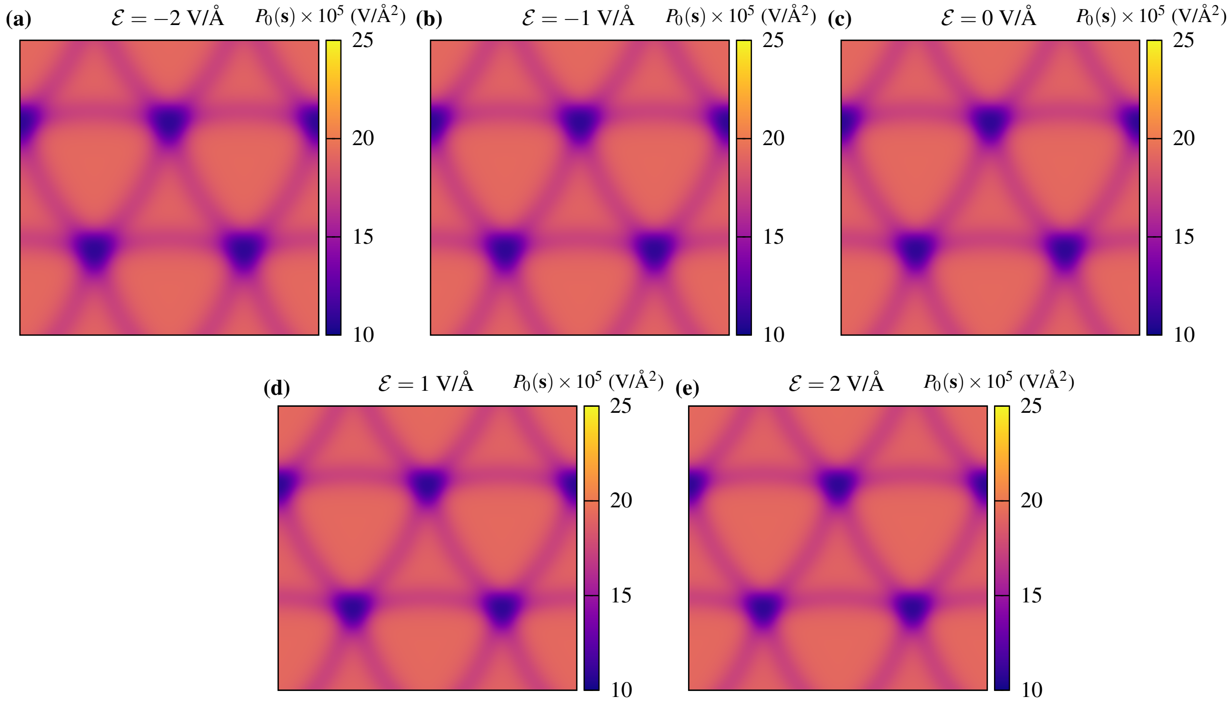


FIG. 21. Lattice relaxtion for 2H-stacked bilayer $MoS_2/MoSe_2$ at a twist angle of $\theta = 0.9^\circ$ for several electric field values.
